# Supplementary material for: Invisible Users: Uncovering End-Users' Requirements for Explainable AI via Explanation Forms and Goals
Source: arXiv:2302.06609 source file (2023-02-15)
Supplement: Supplementary file 1 [file InvisibleUsers_appendix.pdf]

# Invisible Users: Uncovering End-Users' Requirements for Explainable AI via Explanation Forms and Goals

## Appendix: Literature Review, Visual Representations of Explanation Forms, Study Method and Material

Weina Jin<sup>1</sup>      Jianyu Fan<sup>2</sup>      Diane Gromala<sup>2</sup>      Philippe Pasquier<sup>2</sup>  
Ghassan Hamarneh<sup>1</sup>

<sup>1</sup>School of Computing Science, Simon Fraser University

<sup>2</sup>School of Interactive Arts and Technology, Simon Fraser University

In this Appendix, we provide details on the literature review for the development of explanation forms in §1, the visual representations of each explanation form in §2, and the study method and participants' demographic information in §3. We attach the interview material at the end, including the tasks, explanation goals, and explanation forms.

## Contents

|          |                                                                       |          |
|----------|-----------------------------------------------------------------------|----------|
| <b>1</b> | <b>Development of the End-User-Friendly Explanation Forms</b>         | <b>2</b> |
| <b>2</b> | <b>Visual Representations of the Explanation Forms</b>                | <b>2</b> |
| 2.1      | Feature-Based Explanation . . . . .                                   | 2        |
| 2.1.1    | Feature Attribution . . . . .                                         | 2        |
| 2.1.2    | Feature Shape . . . . .                                               | 3        |
| 2.1.3    | Feature Interaction . . . . .                                         | 4        |
| 2.2      | Example-Based Explanation . . . . .                                   | 4        |
| 2.2.1    | Similar Example . . . . .                                             | 4        |
| 2.2.2    | Typical Example . . . . .                                             | 5        |
| 2.2.3    | Counterfactual Example . . . . .                                      | 5        |
| 2.3      | Rule-Based Explanation . . . . .                                      | 5        |
| 2.3.1    | Decision Rule . . . . .                                               | 6        |
| 2.3.2    | Decision Tree . . . . .                                               | 6        |
| 2.4      | Contextual information . . . . .                                      | 6        |
| <b>3</b> | <b>User Study Method</b>                                              | <b>8</b> |
| 3.1      | The Interview Instrument . . . . .                                    | 8        |
| 3.1.1    | Critical Decision-Making Tasks . . . . .                              | 8        |
| 3.1.2    | End Users' Explanation Goals . . . . .                                | 10       |
| 3.1.3    | Creating Visual Representation Cards from Explanation Forms . . . . . | 10       |
| 3.2      | Study Procedure . . . . .                                             | 10       |
| 3.2.1    | Round 1: Interview on Explanation Goals . . . . .                     | 10       |
| 3.2.2    | Round 2: Card Selection and Ranking on Explanation Forms . . . . .    | 12       |
| 3.3      | Participants' Information . . . . .                                   | 13       |

|     |                                     |    |
|-----|-------------------------------------|----|
| 3.4 | Demographic Questionnaire . . . . . | 15 |
| 3.5 | Interview Material . . . . .        | 16 |

# 1 Development of the End-User-Friendly Explanation Forms

The development of the end-user-friendly explanation forms is based on existing XAI techniques in the literature of AI, human-computer interaction (HCI), and information visualization (VIS). We develop the explanation forms by conducting a literature review and examining XAI surveys in the AI, VIS, and HCI domains.

For the literature review, we searched for XAI technique papers using “explainable/interpretable/transparency/ black box” + “AI/machine learning/deep learning” in Google Scholar, IEEE Xplore Digital library, ACM Digital library, and arXiv.org in 2019, and excluded works that did not conduct evaluation on the proposed XAI algorithm.

For the papers included, we labelled the type of their output explanatory information, and identify the requisite technical literacy to understand the output explanatory information. We repeated the process until information “saturated”, i.e., no new explanatory forms were identified.

A total of 66 papers were reviewed and analyzed. We extracted the following information from the included papers: algorithm name (if there is any); the inputs to generate the explanatory model (such as whether it needs access to the training data, the original model parameters); the original model to be explained (model-agnostic vs. model-specific; post-hoc vs. intrinsic); the brief description of the algorithm; the output explanatory information of the XAI model; visualization analysis of the explanatory information (including the explanatory data type, encoding method, and the screenshot of the visualization figures); the evaluation of the XAI method; whether it gives local or global explanations; whether it targets AI developers or/end-users. The list of papers and their extracted information is in the following pages.

The labels revealed 12 primary types of explanatory information: feature attribution, feature shape, feature interaction, concept; decision tree, rule, counterfactual rule; instance, counterfactual instance, prototype, similar example, and clustering. We grouped them into three major categories: explaining based on features, examples, and rules. We also added input, output, performance, and dataset to the explanatory forms as necessary contextual information to make the explanation more complete.

After the primary development of the 12 end-user-friendly explanation forms, we also reviewed the up-to-date related XAI surveys in AI [20, 13, 25, 19, 18, 26, 21, 12, 5, 7], HCI [17, 14, 3, 11, 9], and VIS [4, 24]. Despite some surveys having similar taxonomies based on the explanation representation forms, none of the surveys explicitly summarize the XAI techniques based on end users’ perspective. Therefore, we kept the original structure and categories of the 12 end-user-friendly explanation forms, and updated it with the latest XAI algorithms that can generate such a explanation form.

## 2 Visual Representations of the Explanation Forms

### 2.1 Feature-Based Explanation

#### 2.1.1 Feature Attribution

*Visual representation:* Its visual representations largely depend on the feature data type. For image and text data, overlaying a **saliency map** or color map on the input is the most common visualization. It uses sequential colors to code the fine-grained feature importance score for each individual feature (could be a pixel for image input, a word for text data). For image/video input data, other popular visualizations include using *segmentation masks* or *bounding boxes* on important image objects/parts.

To visualize multiple feature attributions for tabular or text data, a **bar chart** is a typical choice. Variations of the bar chart include waterfall plot, treemap, wrapped bars, packed bars, piled bars, Zvinca plots, and tornado plot. Compared to a bar chart that shows a point estimation of feature importance, a *box plot* can be used to visualize the probabilistic distribution of the feature importance score. Its variations include violin plot and swarm plot that show more detailed data distribution and skewness.

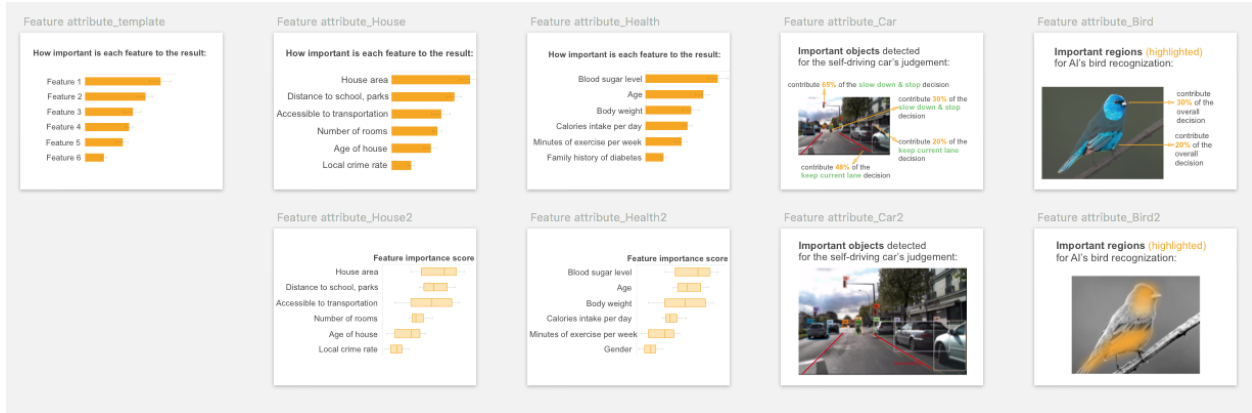

Figure 1: Visual representations of feature attribution. The first column is the template with feature names shown by placeholders. The following columns are the visual representation cards used in the four tasks (House, Health, Car, Bird) in the user study. Different visual variations are shown in the second row.

### 2.1.2 Feature Shape

*Visual representation:* For a continuous feature (such as height, temperature, i.e.: measurement on a scale), a **line chart** is the most common visualization, depicting whether the relationship between the feature and outcome is monotonic, linear, or more complex. The line chart can be accompanied by a scatter plot detailing the position of individual data points.

For a categorical feature (such as gender, season), a *bar chart* can be used.

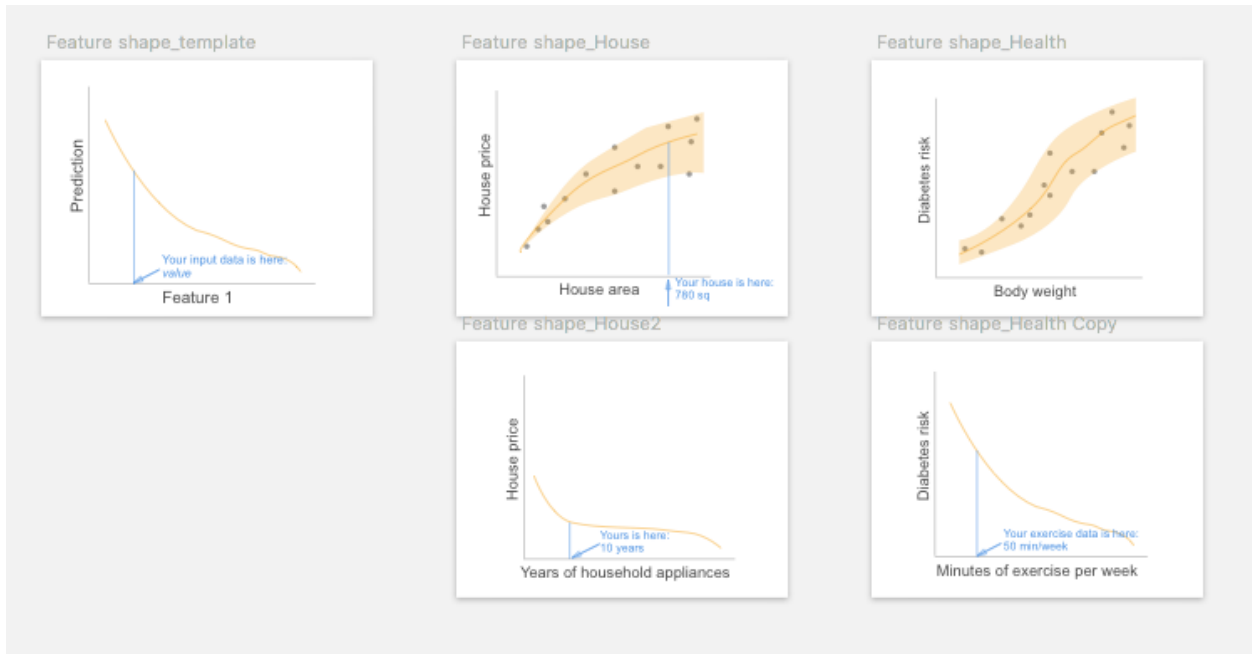

Figure 2: Visual representations of feature shape. The first column is the template with feature names shown by placeholders. The following columns are the visual representation cards used in the two tasks (House, Health) in the user study. Different visual variations are shown in the second row.

### 2.1.3 Feature Interaction

*Visual representation:* **2D or 3D heatmap** is usually used to visualize the combined effect of feature interactions on prediction. Limited by the visualization, a heatmap can show feature interactions for at most three features (using 3D heatmap). More complicated multiple paired feature-feature interactions can be visualized using matrix heatmap, node-link network, or contingency wheel.

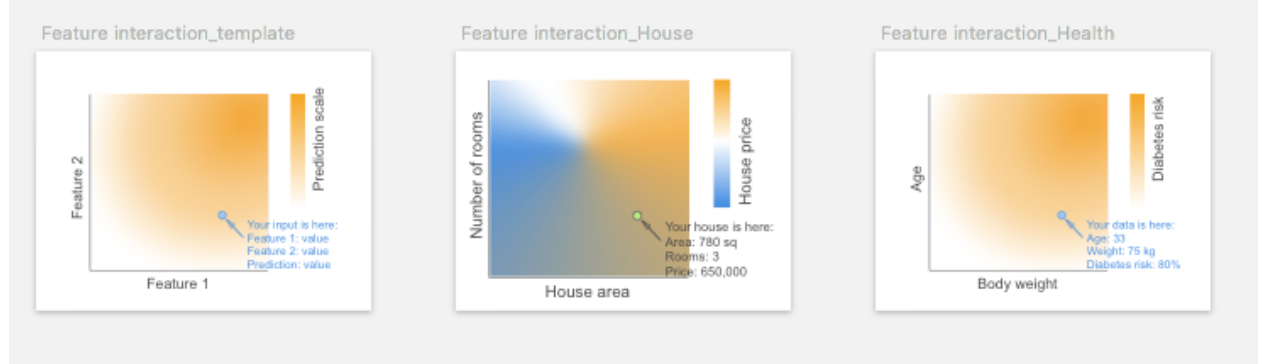

Figure 3: Visual representations of feature interaction. The first column is the template with feature names shown by placeholders. The following columns are the visual representation cards used in the two tasks (House, Health) in the user study.

## 2.2 Example-Based Explanation

### 2.2.1 Similar Example

The differences among similar, typical, and counterfactual examples are listed in Table A1: For a similar example, although it shares *similar features* with the query instance, their predictions may be *the same or different*. Whereas for a counterfactual example, it not only shares *similar features* with the query instance, but also has a *different prediction*. For a typical example, it has *the same prediction* as the query instance, regardless of their features.

| Explanation Form              | Features             | Prediction            |
|-------------------------------|----------------------|-----------------------|
| <b>Similar</b> Example        | similar              | the same or different |
| <b>Typical</b> Example        | similar or different | the same              |
| <b>Counterfactual</b> Example | similar              | different             |

Table A1: **Distinctions among the three example-based explanation forms** by comparing their features and prediction with the query instance.

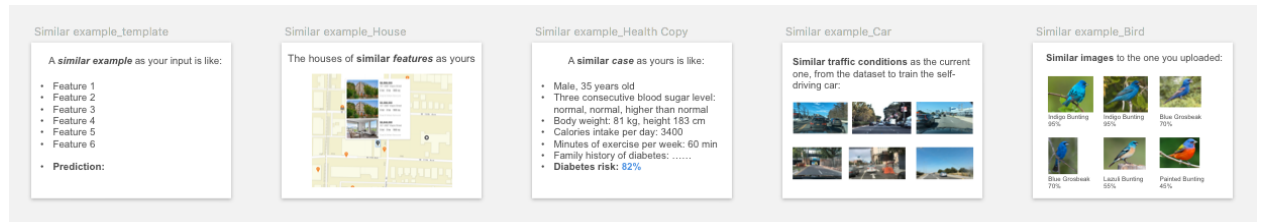

Figure 4: Visual representations of similar example. The first column is the template with feature names shown by placeholders. The following columns are the visual representation cards used in the four tasks (House, Health, Car, Bird) in the user study.

## 2.2.2 Typical Example

*Visual representation:* For similar and typical examples, it is straightforward to show several examples with their corresponding predictions.

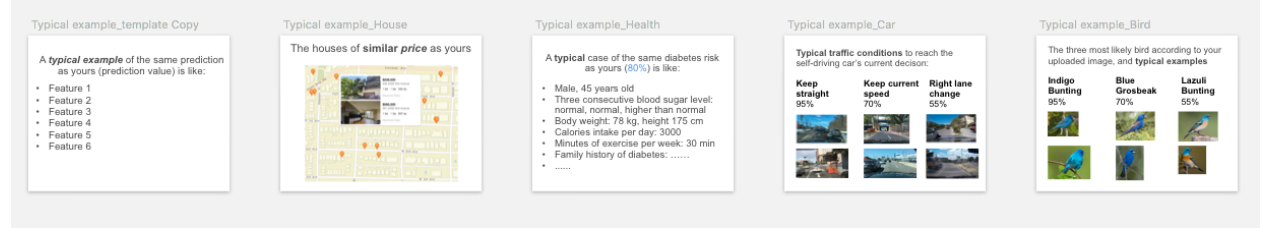

Figure 5: Visual representations of typical example. The first column is the template with feature names shown by placeholders. The following columns are the visual representation cards used in the four tasks (House, Health, Car, Bird) in the user study.

## 2.2.3 Counterfactual Example

We noted that counterfactual explanations can also be expressed as counterfactual features or rules. However, a counterfactual feature/rule can not be a standalone explanation in an XAI system, they must reside within a certain context by assuming all other features are constant. To make the explanation information complete, we include the counterfactual explanation in the form of example.

*Visual representation:* Counterfactual examples can be shown as two instances and their predictions, with their **counterfactual/contrasting features highlighted**, or a **transition** from one instance to the other by gradually changing the counterfactual features.

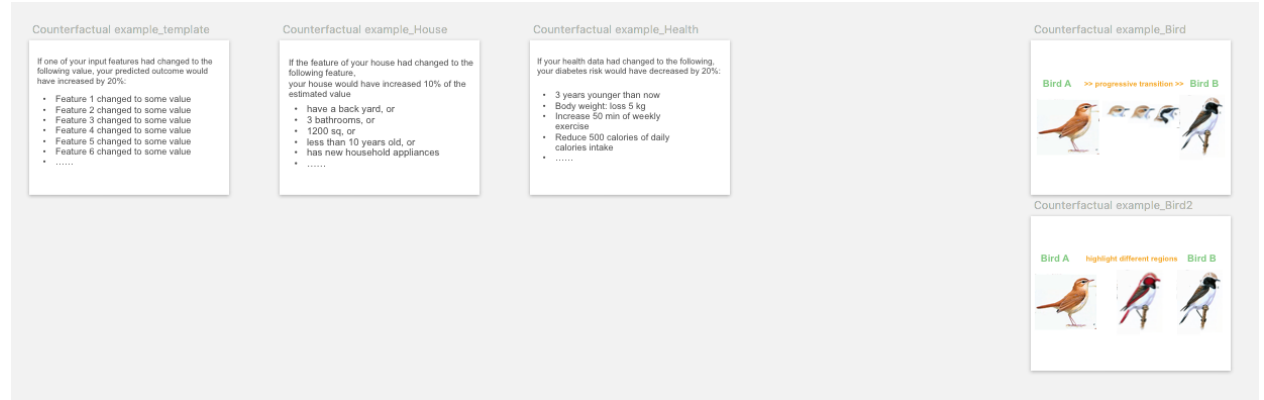

Figure 6: Visual representations of counterfactual example. The first column is the template with feature names shown by placeholders. The following columns are the visual representation cards used in the three tasks (House, Health, Bird) in the user study. We did not include a counterfactual example for the Car task, therefore we leave the column black. Different visual variations are shown in the second row.

## 2.3 Rule-Based Explanation

We note decision rule and decision tree actually carry similar explanation information. However, since they are usually generated by different XAI algorithms, and their representation formats (text vs. diagram) are different to users, we included them as two separate explanation forms.

### 2.3.1 Decision Rule

*Visual representation:* Decision rules are usually represented using **text**. Other representing formats include table [8] or matrix [16] to align, read, and compare rule clauses more easily.

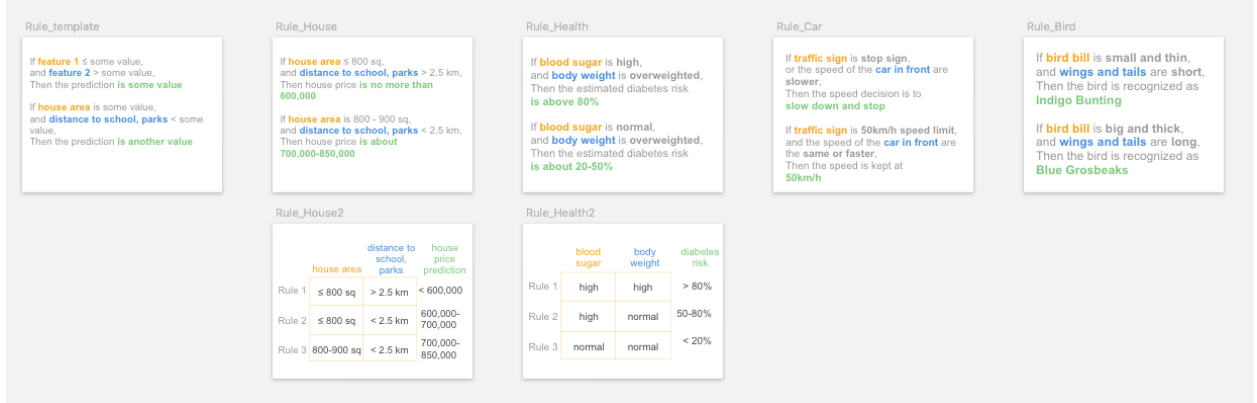

Figure 7: Visual representations of decision rule. The first column is the template with feature names shown by placeholders. The following columns are the visual representation cards used in the four tasks (House, Health, Car, Bird) in the user study. Different visual variations are shown in the second row.

### 2.3.2 Decision Tree

*Visual representation:* The most common representation is to use a node-link **tree diagram**. Other visual representations to show the hierarchical structure include treemap, cladogram, hyperbolic tree, dendrogram, and flow chart.

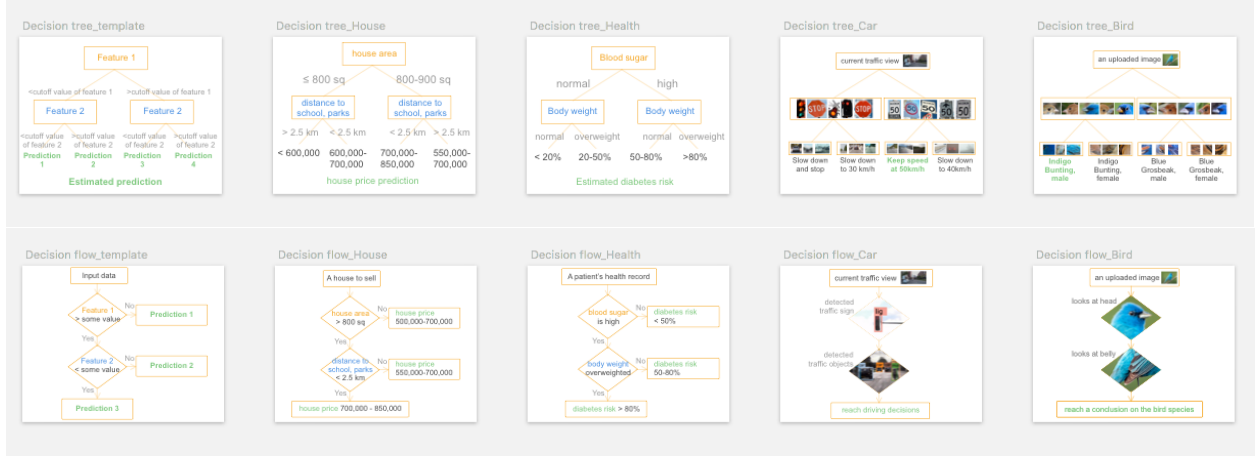

Figure 8: Visual representations of decision tree (1st row) and decision flow (2nd row). The first column is the template with feature names shown by placeholders. The following columns are the visual representation cards used in the four tasks (House, Health, Car, Bird) in the user study.

## 2.4 Contextual information

To provide necessary context and background for a more complete explanation, we additionally include contextual information in the end user-friendly explanation forms, include:

**Input  $x$ .**

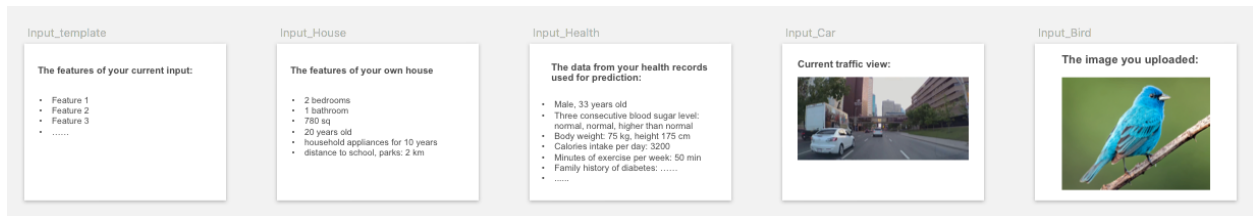

Figure 9: Visual representations of input. The first column is the template with feature names shown by placeholders. The following columns are the visual representation cards used in the four tasks (House, Health, Car, Bird) in the user study.

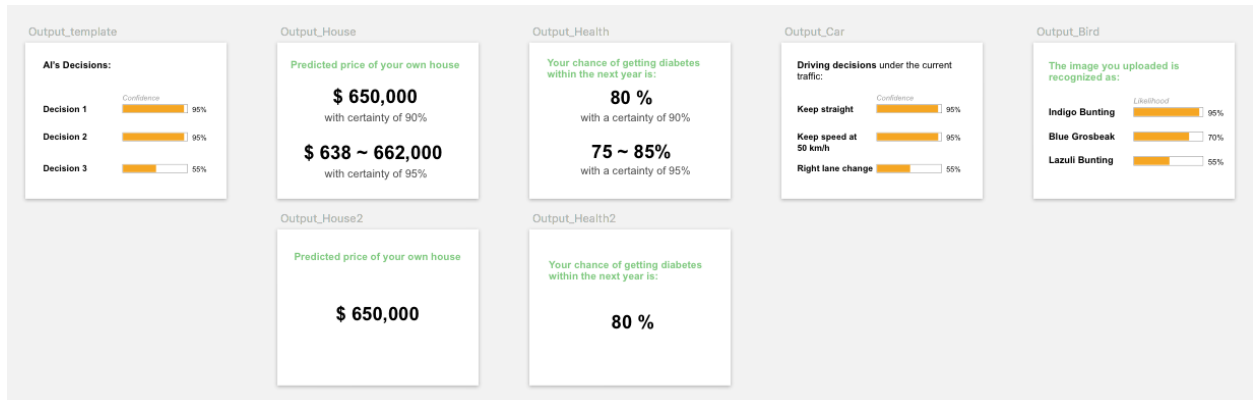

Figure 10: Visual representations of output. The first column is the template shown using placeholders. The following columns are the visual representation cards used in the four tasks (House, Health, Car, Bird) in the user study. Different visual variations are shown in the second row.

### Output $y$ .

**Performance:** Model's performance metrics (such as prediction accuracy, confusion matrix, ROC, mean squared error) help end users to judge a model's overall decision quality and set a proper expectation on model's capability.

**Dataset:** It is the proper description of the training and validation dataset, such as data distribution, and how the data were collected.

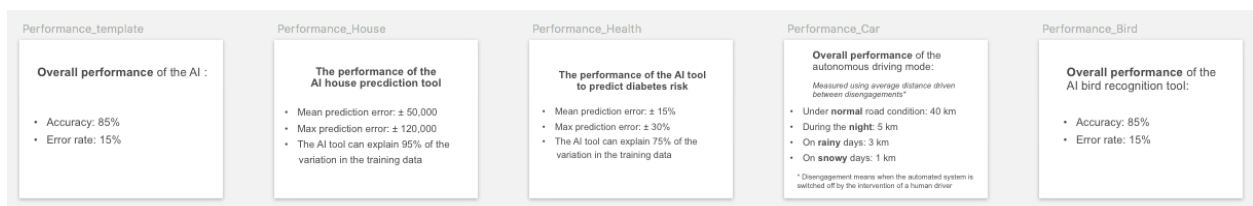

Figure 11: Visual representations of performance. The first column is the template. The following columns are the visual representation cards used in the four tasks (House, Health, Car, Bird) in the user study.

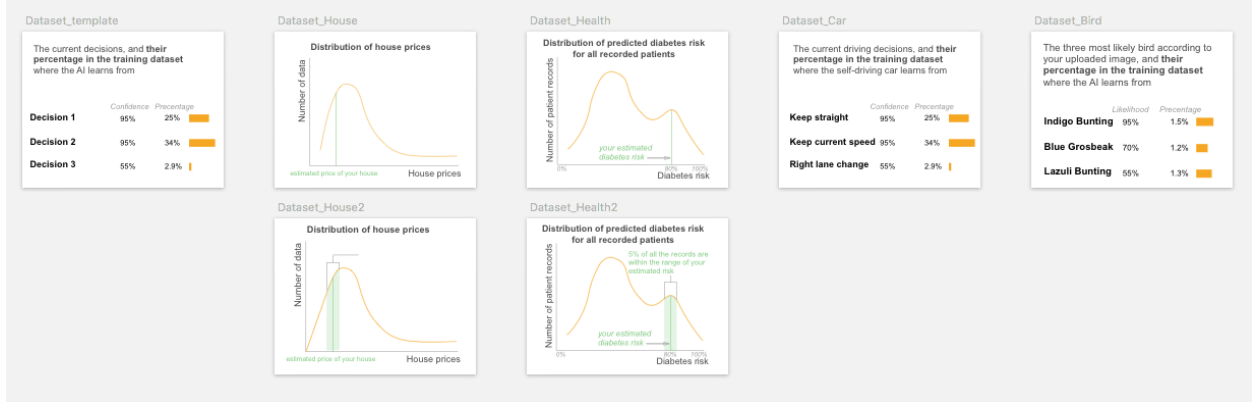

Figure 12: Visual representations of dataset. The first column is the template shown using placeholders. The following columns are the visual representation cards used in the four tasks (House, Health, Car, Bird) in the user study. Different visual variations are shown in the second row.

### 3 User Study Method

#### 3.1 The Interview Instrument

##### 3.1.1 Critical Decision-Making Tasks

We focus the scope of the study on AI-assisted critical decision-support tasks, where explanations have high utility as shown in previous research [6, 15, 10], and AI could not be delegated to have full automation because of the high-stakes nature of the tasks and the liability issue. In this study phase, we did not include domain experts. Therefore, we deliberately designed the tasks so that decisions can be made based on common sense without requiring domain knowledge. We designed four decision-making tasks reflecting the diversity of AI-supported critical decision-making. They are:

1. **House** task: users use AI to get a proper estimate of their house price.
2. **Health** task: users use AI to predict his/her diabetes risk.
3. **Car** task: users decide whether to buy an autonomous driving vehicle.
4. **Bird** task: users use AI bird recognition tool to prepare for an important biology exam.

The four tasks are critical decision-making scenarios, because their decisions have significant consequences on one's health and life (Health and Car Task), finance (House Task), or education (Bird Task). The corresponding datasets of the four tasks are publicly available (Table A2), so that the resultant low-fidelity paper-based AI prototypes from this user study can be actualized as high-fidelity functional prototypes for task-specific studies in future work.

| <i>AI-Assisted Critical Decision-Making Tasks</i> | <b>HOUSE TASK</b><br><br>Sell a house<br>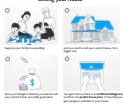 | <b>HEALTH TASK</b><br><br>Check diabetes risk<br>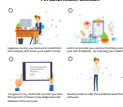                   | <b>CAR TASK</b><br><br>Buy a self-driving car<br>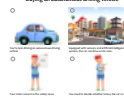                                                                                        | <b>BIRD TASK</b><br><br>Prepare for exam<br>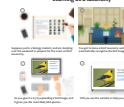 |
|---------------------------------------------------|----------------------------------------------------------------------------------------------------------------------------|------------------------------------------------------------------------------------------------------------------------------------------------------|----------------------------------------------------------------------------------------------------------------------------------------------------------------------------------------------------------------------------|---------------------------------------------------------------------------------------------------------------------------------|
| <i>Explanation Goals</i>                          | <b>Calibrate Trust</b>                                                                                                     | You doubt whether to trust the AI tool or not                                                                                                        | n/a                                                                                                                                                                                                                        | You don't know whether to trust the results from the website or not                                                             |
|                                                   | <b>Ensure Safety</b>                                                                                                       | n/a                                                                                                                                                  | n/a                                                                                                                                                                                                                        | n/a                                                                                                                             |
|                                                   | <b>Detect Bias</b>                                                                                                         | n/a                                                                                                                                                  | You doubt whether the software will perform the same among people with different gender, age, or ethnicity group                                                                                                           | n/a                                                                                                                             |
|                                                   | <b>Unexpected Prediction: Disagreement with AI</b>                                                                         | AI's prediction aligns/does not align with your own estimation                                                                                       | You maintain good health with no major diseases or a family history of diabetes/Diabetes tends to run in your family, and you're afraid of getting it someday, and AI predicts your chance of getting diabetes is low/high | You notice the car sometimes drives much slower than the expected speed limit                                                   |
|                                                   | <b>Differentiation Similar Instances</b>                                                                                   | n/a                                                                                                                                                  | n/a                                                                                                                                                                                                                        | The results sometimes do not align with your knowledge                                                                          |
|                                                   | <b>Learn from AI</b>                                                                                                       | n/a                                                                                                                                                  | n/a                                                                                                                                                                                                                        | In the exam, you need to write a short statement to differentiate different birds                                               |
|                                                   | <b>Improve the Predicted Outcome</b>                                                                                       | n/a                                                                                                                                                  | n/a                                                                                                                                                                                                                        | Is it a good tool to improve your learning and help you know more about bird taxonomy?                                          |
|                                                   | <b>Communicate with Stakeholders</b>                                                                                       | You need to decide whether to do a renovation or replacement of appliances to increase your house value, and which action is the most cost-effective | You want to know how to adjust your lifestyle accordingly to lower the risk of diabetes                                                                                                                                    | n/a                                                                                                                             |
|                                                   | <b>Generate Reports</b>                                                                                                    | You need to communicate your decision with your family                                                                                               | You need to need to inform family members and consult your doctor                                                                                                                                                          | n/a                                                                                                                             |
|                                                   | <b>Multi-Objectives Trade-Off</b>                                                                                          | n/a                                                                                                                                                  | n/a                                                                                                                                                                                                                        | n/a                                                                                                                             |
| <i>ML problem type</i>                            | Regression                                                                                                                 | Regression                                                                                                                                           | Classification                                                                                                                                                                                                             | Classification                                                                                                                  |
| <i>Input data type</i>                            | Tabular data                                                                                                               | Tabular/sequential data                                                                                                                              | Image/video data                                                                                                                                                                                                           | Image data                                                                                                                      |
| <i>Available dataset</i>                          | Boston housing [2]                                                                                                         | Diabetes dataset [1]                                                                                                                                 | BDD100K [23]                                                                                                                                                                                                               | CUB-200 dataset [22]                                                                                                            |

Table A2: The four tasks and their explanation goals used in the user study.

### 3.1.2 End Users’ Explanation Goals

Even for the same user and task, end users’ explanation goals, i.e.: the trigger point or motivation to check the explanation of an AI system, may vary in different contexts or usage scenarios. In our study, we aim to capture the fine-grained details of end users’ requirements for different explanation goals. We instantiated the identified explanation goals for each task, trying to cover as many explanation goals as we can. Table A2 shows the explanation task and their accompanying scenarios describing an explanation goal.

### 3.1.3 Creating Visual Representation Cards from Explanation Forms

We instantiated the explanation forms as low-fidelity visual cards for each task, based on their visual representations. We illustrate this process below:

1. **Create visual card templates** We started by creating visual representation templates of the explanation forms. We selected the most common visualizations, based on the summarized visual representations in Section 2. For example, we used bar chart and color map to visualize feature attribution for tabular and image data respectively. Each individual card shows one visual representation of an explanation form. For some explanation forms (such as feature attribution and counterfactual example), we created multiple cards with different variations of their visual representations.
2. **Extract features as content placeholder** We then manually extracted several interpretable features given the AI task. For instance, in the house price prediction task, we extracted features of house size, age, etc. In the self-driving car task, we extracted saliency objects such as traffic signs, road markers, cars, and pedestrians. As a quick prototyping, the feature content may not necessarily reflect the real content generated by XAI algorithms. They mainly serve as content placeholders.
3. **Fill the visual card templates with content placeholders** The extracted features were then used to fill in the visual card templates. The final visual representation cards are shown as figures in Section 2.

After interviewing the first five participants, we revised some visual cards based on participants’ feedback. For instance, we indicated the position of the input data point on the feature shape and feature interaction cards. We also removed several variations of the cards (such as using a table to represent rules) since participants found them difficult to interpret.

## 3.2 Study Procedure

The study procedure consists of two rounds. **Round 1** is to familiarize participants with the tasks and explanation goals, and to understand end users’ explanation goals for XAI before showing them the visual cards of the explanation forms. **Round 2** is the selection & ranking to understand users’ interpretations and requirements for the explanation forms.

### 3.2.1 Round 1: Interview on Explanation Goals

We began the user study by introducing the researchers and the aim of the study, and went through the study consent form with the participant. The interview started after gaining the participant’s written consent.

**Task** We first introduced an AI-assisted task to participants. The choice of the task was determined by a pre-generated random sequence. The task was presented as a storyboard color-printed on paper. Fig. 13 shows an example of the storyboard of the Health task. The researcher asked the participant to assume s/he was the character in the story context, and went through the task context with the participant by reading the text on the storyboard.

**Explanation Goal** After confirming that the participant had no questions and fully understood the current task, the research then randomly selected an explanation goal under the task context. The explanation goal was also shown as a storyboard picture, and the researcher read the text on the picture to introduce the explanation goal. Figure 14 gives an example of an explanation goal of *unexpected*. For each explanation goal, the researcher asked the participants whether they accept AI as decision-support, and need

## Personal health decision

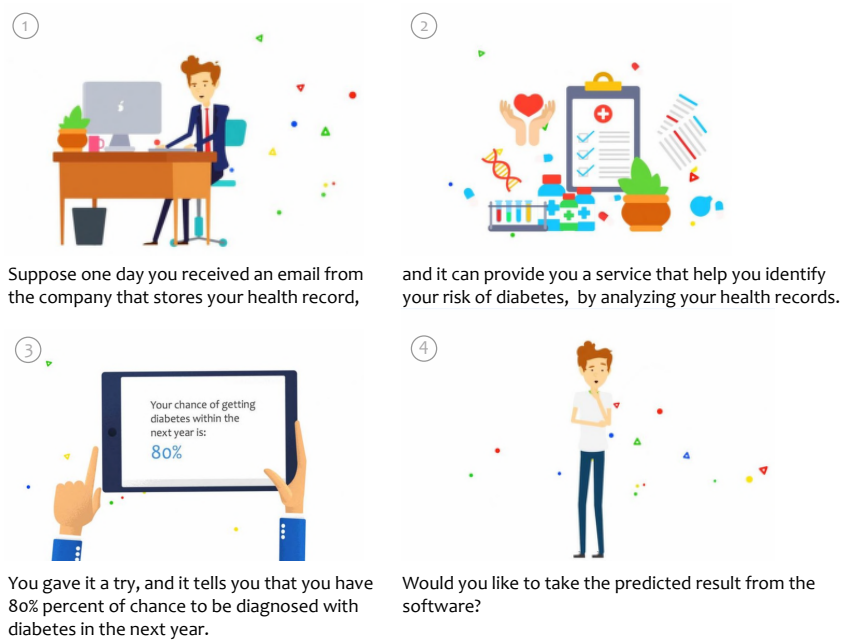

Figure 13: The interview storyboard of the Health task in the user study

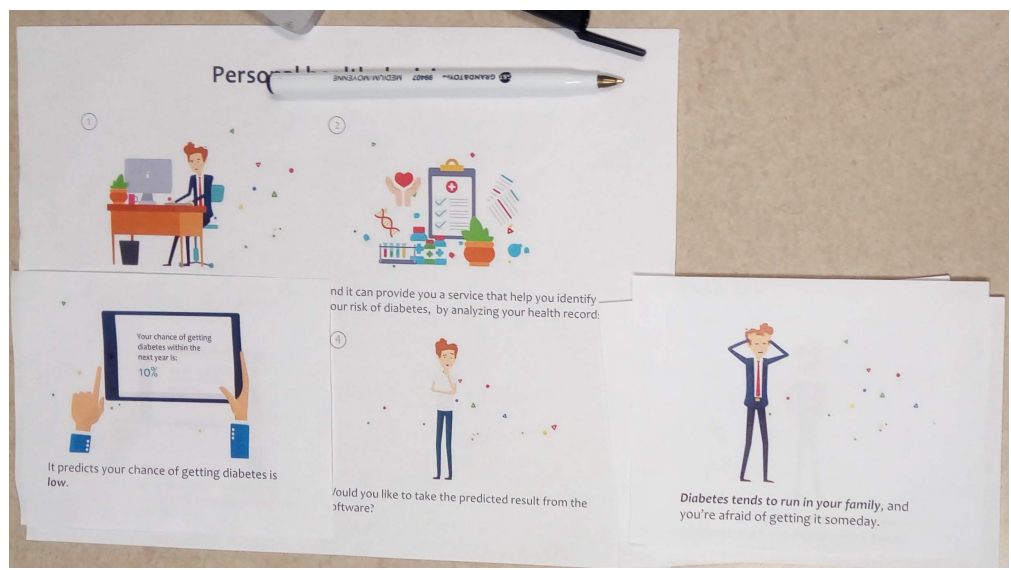

Figure 14: The explanation goal of **unexpected** in the Health task context. The end user may expect to have a high risk of diabetes due to family history. However, AI predicts the risk is only 10% which may not align with the user's expectation.

AI to explain its decision. If explanations were needed, the researcher then asked what explanations/further information they request.

After discussing all explanation goals for one task, the participant entered Round 2: card selection & ranking, which is detailed in the next subsection.

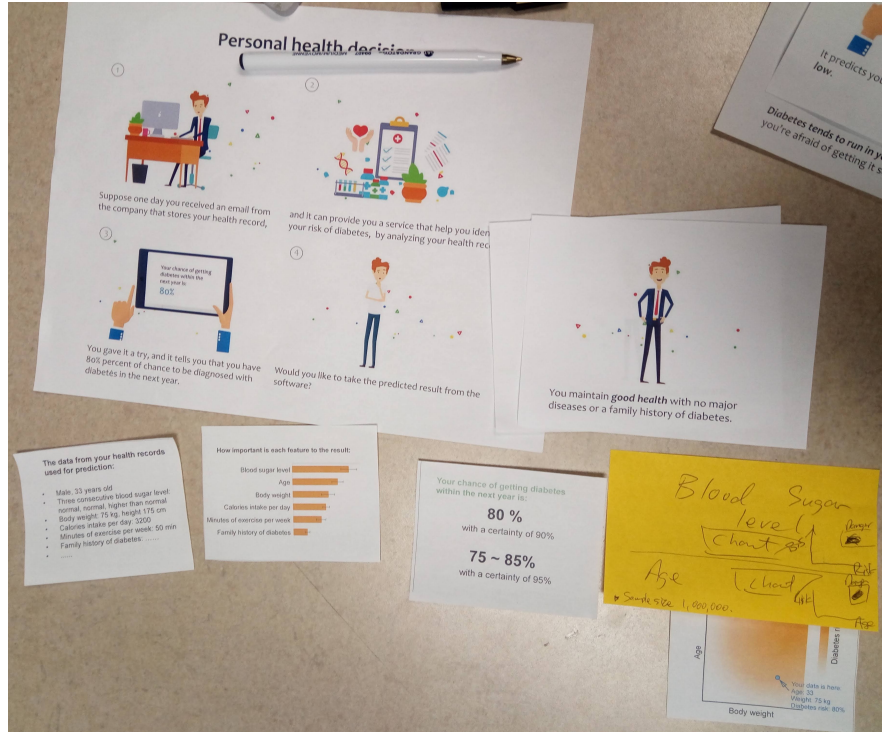

Figure 15: **The card selection & ranking result from one participant.** Given the task and explanation goal, the participant selected and ranked the visual cards from left to right according to their usefulness to the given explanation goal. She also sketched to improve the last card on feature interaction.

After completing one task, if the duration of the interview was less than 30 minutes, the participants were assigned to another task and underwent the same two-round interview procedure. At the end of the interview, the participants filled out a demographic questionnaire (Section 3.4). The study session duration is  $67.9 \pm 18.8$  (Mean  $\pm$  SD) minutes (Median: 67 min, Range: 41 - 120 min, each participant's specific data are detailed in Table 3.3). We audio-recorded the interviews, made observational notes on the card selection & ranking process, and took pictures of the card selection & ranking results. All study materials including the storyboards of tasks and explanation goals, and visual representation cards of explanation forms are listed at the end of this document.

### 3.2.2 Round 2: Card Selection and Ranking on Explanation Forms

For each decision-making task, the participants first revisited the task. Then the researcher gave a short tutorial of the explanation forms by walking through the visual cards and explaining the information on a card. In this process, the participant could ask questions if s/he did not understand or needed clarification. S/he could also comment on each card. Before moving on to the next step, we asked the participant and made sure they had no questions on these cards.

After confirming the participant fully understand the content of the cards, for each explanation goal, the researcher asked participants to select, rank, and combine the visual cards that they found were the most useful ones and could meet their current explanation goals. The participants could comment on any card anytime during this process. They could also modify the existing cards, or sketch on blank cards to create new visual cards, and add the newly created/modified cards to the card selection & ranking. After ranking the cards, they were asked to comment on why they selected or did not select a card, and their rationals for making such a ranking. After the card selection & ranking, they were asked whether the combination of cards would fulfill their explanation goals.

### 3.3 Participants' Information

| Participant number | Age | Sex | Education level     | Major or Industry                   | AI familiarity                                                              | AI attitudes                     | Tasks                    | Interview duration (min) |
|--------------------|-----|-----|---------------------|-------------------------------------|-----------------------------------------------------------------------------|----------------------------------|--------------------------|--------------------------|
| P01                | 38  | M   | Bachelor            | computer science                    | program but not in AI                                                       | interested                       | House; Health; Car; Bird | 120                      |
| P02                | 26  | M   | PhD                 | HCI                                 | program but not in AI                                                       | concerned; interested; excited   | Health; Bird             | 90                       |
| P03                | 29  | F   | PhD                 | HCI                                 | use AI (Google) to re-minders/navigation/daily use/play music or video etc. | interested                       | House; Car               | 74                       |
| P04                | 28  | M   | Master              | HCI                                 | program but not in AI                                                       | concerned; interested; excited   | House; Car               | 94                       |
| P05                | 40  | F   | Trade               | editing                             | heard                                                                       | concerned; interested; excited   | Car; Bird                | 46                       |
| P06                | 21  | F   | Some college credit | psychology                          | use AI (Google home) to play music                                          | concerned; skeptical; interested | Health; Bird             | 76                       |
| P07                | 62  | M   | Bachelor            |                                     |                                                                             |                                  | House; Car               | 64                       |
| P08                | 22  | F   | High school         | computer science                    | program but not write AI code                                               | excited                          | Health; Bird             | 55                       |
| P09                | 40  | M   | Bachelor            | Business development and sales (IT) | use AI (Google navigator) to traffic and directions                         | excited                          | Car; Bird                | 51                       |
| P10                | 19  | M   | High school         | cooking                             | heard                                                                       | neutral                          | House; Bird              | 54                       |
| P11                | 30  | F   | Bachelor            | IT                                  | program but not write AI code                                               | interested                       | House; Bird              | 76                       |
| P12                | 48  | F   | High school         |                                     | heard                                                                       | neutral                          | House; Bird              | 74                       |
| P13                | 53  | M   | Bachelor            | customer service                    | heard                                                                       | concerned; skeptical             | Health; Car              | 69                       |
| P14                | 47  | M   | Some college credit | healthcare-sterilization work       | never                                                                       | interested                       | House; Bird              | 55                       |

| Participant number | Age | Sex | Education level     | Major or Industry                                                          | AI familiarity                                                  | AI attitudes                                       | Tasks          | Interview duration (min) |
|--------------------|-----|-----|---------------------|----------------------------------------------------------------------------|-----------------------------------------------------------------|----------------------------------------------------|----------------|--------------------------|
| P15                | 73  | M   | Professional        | retired                                                                    | heard                                                           | skeptical                                          | Car            | 81                       |
| P16                | 34  | F   | Professional        | law                                                                        | heard                                                           | concerned;<br>interested;<br>excited               | Health         | 67                       |
| P17                | 70  | M   | Bachelor            | retired                                                                    | heard                                                           | neutral                                            | Health;<br>Car | 47                       |
| P18                | 27  | M   | Some college credit | General studies and legal studies                                          | heard                                                           | skeptical;<br>neutral;<br>excited                  | Bird           | 41                       |
| P19                | 35  | F   | Bachelor            | Government or social services (employment services for indigenous peoples) | heard                                                           | concerned;<br>skeptical;<br>interested;<br>excited | House;<br>Car  | 42                       |
| P20                | 30  | M   | Bachelor            | Food industry                                                              | heard                                                           | concerned;<br>skeptical;<br>interested;<br>excited | House          | 58                       |
| P21                | 26  | F   | Bachelor            | Interior designer                                                          | use AI (chatting with clients)                                  | concerned;<br>interested;<br>excited               | Car            | 60                       |
| P22                | 23  | F   | Some college credit | Student (RMT); Work (hospitality (restaurant))                             | heard                                                           | concerned;<br>skeptical;<br>excited                | Health         | 69                       |
| P23                | 31  | M   | Master              | Accountant                                                                 | use AI (google Home) to preferred music/movie                   | excited                                            | Health         | 72                       |
| P24                | 41  | M   | Bachelor            | Financial industry                                                         | use AI (investment software) to help drive investment decisions | excited                                            | Health         | 69                       |
| P25                | 72  | M   | Master              | retired                                                                    | heard                                                           | concerned;<br>interested;<br>excited               | Health         | 112                      |
| P26                | 70  | F   | Bachelor            | retired                                                                    | heard                                                           | skeptical;<br>interested                           | Bird           | 52                       |
| P27                | 28  | F   | Bachelor            | hospitality                                                                | heard                                                           | interested                                         | Car            | 45                       |
| P28                | 28  | M   | Trade               | Marlcotins sale                                                            | heard                                                           | interested                                         | Health         | 88                       |

| Participant number | Age | Sex | Education level | Major or Industry                                     | AI familiarity                | AI attitudes                   | Tasks  | Interview duration (min) |
|--------------------|-----|-----|-----------------|-------------------------------------------------------|-------------------------------|--------------------------------|--------|--------------------------|
| P29                | 43  | F   | Bachelor        | Project management in construction (currently no job) | heard                         | concerned; interested; excited | House  | 67                       |
| P30                | 24  | F   | Master          | Computer science                                      | program but not write AI code | concerned                      | House  | 83                       |
| P31                | 25  | F   | Bachelor        | psychology office worker                              | heard                         | interested                     | Health | 65                       |
| P32                | 39  | F   | Bachelor        | car insurance                                         | heard                         | excited                        | Car    | 59                       |

### 3.4 Demographic Questionnaire

1. Your age: \_\_\_\_\_

☐ prefer not to disclose

2. Your gender:

☐ Female

☐ Male

☐ Other

3. What is the highest degree or level of school you have completed or currently enrolled?

☐ No schooling completed

☐ Nursery school to 8th grade

☐ Some high school, no diploma

☐ High school graduate, diploma or the equivalent (for example: GED)

☐ Some college credit, no degree

☐ Trade/technical/vocational training

☐ Bachelor's degree

☐ Master's degree

☐ Professional degree (e.g. MD, JD)

☐ Doctorate degree (PhD)

4. If you are a student, what is your major? If you are working, what is your current work industry?

5. What is your understanding of artificial intelligence (AI)?

☐ I have never heard of AI before

☐ I only hear of AI from the news, friends, etc.

☐ I use AI in my work or life. If so, please specify what kind of AI do you use: \_\_\_\_\_, to accomplish what tasks: \_\_\_\_\_

☐ I can program, but I can not write AI code

☐ I can write AI code

6. What is your opinion on incorporating AI technology into our everyday decision-making scenarios? (you can select multiple choices)

☐ I am not interested in AI, and I do not pay attention to it

☐ I am concerned about the prevalence of AI (e.g.: it will take over many people's job; it's a threat to human beings)

☐ I am skeptical of the incorporation of AI technology, but I would like to learn more about it

☐ I am neutral regarding the incorporation of AI technology

- ☐ I am interested in the incorporation of AI, and willing to know more about it
- ☐ I am excited to use AI to improve my work and life

### 3.5 Interview Material

We attach the interview material used in the study at the end of the Appendix, including:

1. The four tasks shown as storyboards;
2. The explanation goals shown as storyboards;
3. The explanation forms shown as cards.

## References

- [1] Diabetes Prediction Dataset, 2020. Accessed: 2020-09-10.
- [2] The Boston Housing Dataset, 2020. Accessed: 2020-09-10.
- [3] Ashraf Abdul, Jo Vermeulen, Danding Wang, Brian Y. Lim, and Mohan Kankanhalli. Trends and trajectories for explainable, accountable and intelligible systems: An hci research agenda. In *Proceedings of the 2018 CHI Conference on Human Factors in Computing Systems*, CHI '18, page 1–18, New York, NY, USA, 2018. Association for Computing Machinery.
- [4] Gulsum Alicioglu and Bo Sun. A survey of visual analytics for explainable artificial intelligence methods. *Computers & Graphics*, 102:502–520, 2022.
- [5] Vijay Arya, Rachel K. E. Bellamy, Pin-Yu Chen, Amit Dhurandhar, Michael Hind, Samuel C. Hoffman, Stephanie Houde, Q. Vera Liao, Ronny Luss, Aleksandra Mojsilović, Sami Mourad, Pablo Pedemonte, Ramya Raghavendra, John Richards, Prasanna Sattigeri, Karthikeyan Shanmugam, Moninder Singh, Kush R. Varshney, Dennis Wei, and Yunfeng Zhang. One explanation does not fit all: A toolkit and taxonomy of ai explainability techniques, 2019.
- [6] Andrea Bunt, Matthew Lount, and Catherine Lauzon. Are explanations always important? In *Proceedings of the 2012 ACM international conference on Intelligent User Interfaces - IUI '12*, page 169, New York, New York, USA, 2012. ACM Press.
- [7] Diogo V. Carvalho, Eduardo M. Pereira, and Jaime S. Cardoso. Machine learning interpretability: A survey on methods and metrics. *Electronics*, 8(8), 2019.
- [8] Federica Di Castro and Enrico Bertini. Surrogate Decision Tree Visualization, 2019.
- [9] Larissa Chazette, Jil Klünder, Merve Balci, and Kurt Schneider. How can we develop explainable systems? insights from a literature review and an interview study. In *Proceedings of the International Conference on Software and System Processes and International Conference on Global Software Engineering*, ICSSP'22, page 1–12, New York, NY, USA, 2022. Association for Computing Machinery.
- [10] Finale Doshi-Velez and Been Kim. Towards A Rigorous Science of Interpretable Machine Learning. feb 2017.
- [11] Juliana J. Ferreira and Mateus S. Monteiro. What Are People Doing About XAI User Experience? A Survey on AI Explainability Research and Practice. pages 56–73. Springer, Cham, jul 2020.
- [12] Riccardo Guidotti, Anna Monreale, Salvatore Ruggieri, Franco Turini, Fosca Giannotti, and Dino Pedreschi. A Survey of Methods for Explaining Black Box Models. *ACM Comput. Surv.*, 51(93), 2018.
- [13] Riccardo Guidotti, Anna Monreale, Salvatore Ruggieri, Franco Turini, Fosca Giannotti, and Dino Pedreschi. A survey of methods for explaining black box models. *ACM Comput. Surv.*, 51(5), aug 2018.

- [14] Q. Vera Liao and Kush R. Varshney. Human-centered explainable AI (XAI): from algorithms to user experiences. *CoRR*, abs/2110.10790, 2021.
- [15] Brian Y. Lim and Anind K. Dey. Assessing demand for intelligibility in context-aware applications. In *Proceedings of the 11th international conference on Ubiquitous computing - Ubicomp '09*, page 195, New York, New York, USA, 2009. ACM Press.
- [16] Yao Ming, Huamin Qu, and Enrico Bertini. RuleMatrix: Visualizing and Understanding Classifiers with Rules. *IEEE Transactions on Visualization and Computer Graphics*, 25(1):342–352, jan 2019.
- [17] Sina Mohseni, Niloofar Zarei, and Eric D. Ragan. A multidisciplinary survey and framework for design and evaluation of explainable ai systems. *ACM Trans. Interact. Intell. Syst.*, 11(3–4), aug 2021.
- [18] Ingrid Nunes and Dietmar Jannach. A systematic review and taxonomy of explanations in decision support and recommender systems. *User Modeling and User-Adapted Interaction*, 27(3-5):393–444, 2017.
- [19] Gabrielle Ras, Ning Xie, Marcel van Gerven, and Derek Doran. Explainable deep learning: A field guide for the uninitiated. *J. Artif. Int. Res.*, 73, may 2022.
- [20] Cynthia Rudin, Chaofan Chen, Zhi Chen, Haiyang Huang, Lesia Semenova, and Chudi Zhong. Interpretable machine learning: Fundamental principles and 10 grand challenges. *Statistics Surveys*, 16:1–85, 2022.
- [21] Daniel S. Weld and Gagan Bansal. The challenge of crafting intelligible intelligence. *Communications of the ACM*, 62(6):70–79, mar 2019.
- [22] P. Welinder, S. Branson, T. Mita, C. Wah, F. Schroff, S. Belongie, and P. Perona. Caltech-UCSD Birds 200. Technical Report CNS-TR-2010-001, California Institute of Technology, 2010.
- [23] Fisher Yu, Wenqi Xian, Yingying Chen, Fangchen Liu, Mike Liao, Vashisht Madhavan, and Trevor Darrell. BDD100K: A diverse driving video database with scalable annotation tooling. *CoRR*, abs/1805.04687, 2018.
- [24] Rulei Yu and Lei Shi. A user-based taxonomy for deep learning visualization. *Visual Informatics*, 2(3):147–154, 2018.
- [25] Quanshi Zhang and Song-Chun Zhu. Visual Interpretability for Deep Learning: a Survey. feb 2018.
- [26] Yu Zhang, Peter Tiño, Aleš Leonardis, and Ke Tang. A survey on neural network interpretability, 2021.

# Selling your house

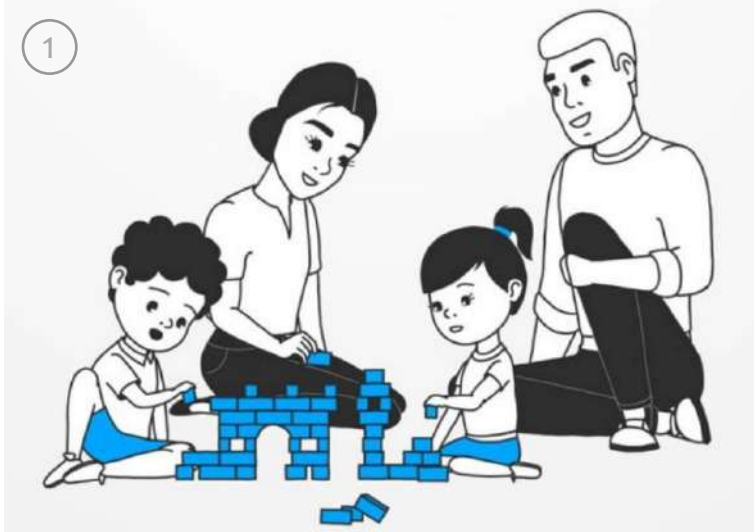

Suppose your family is expanding

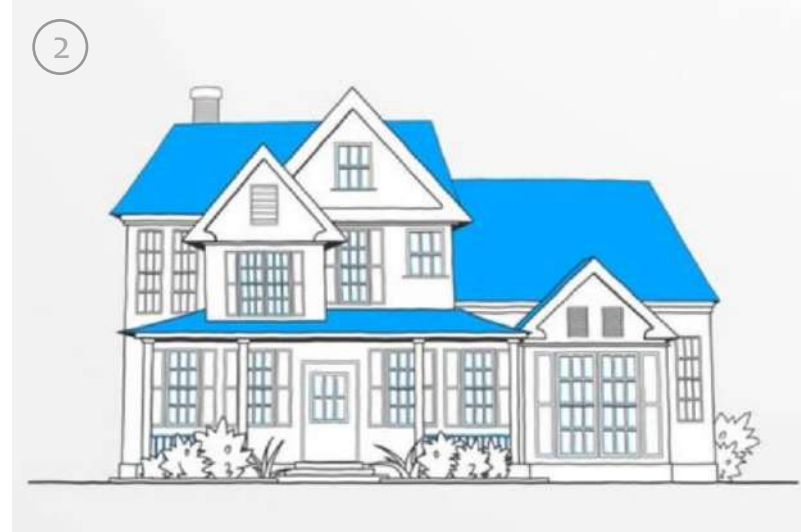

and you need to sell your current house, for a bigger one.

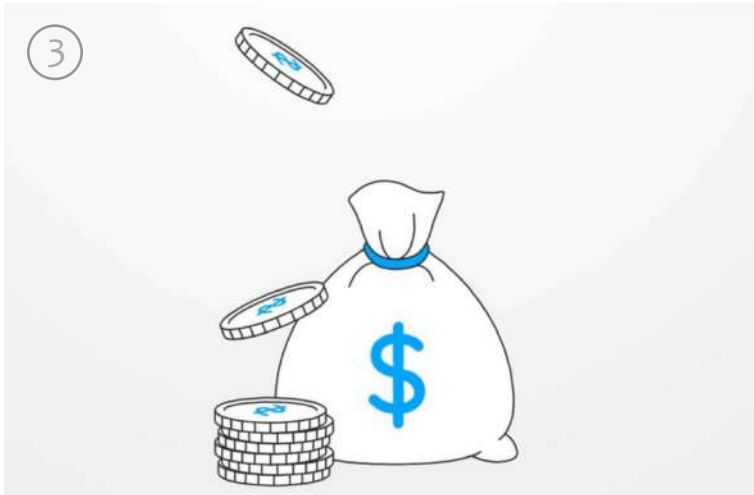

Since your budget is limited, you need to sell your current house at a really good price

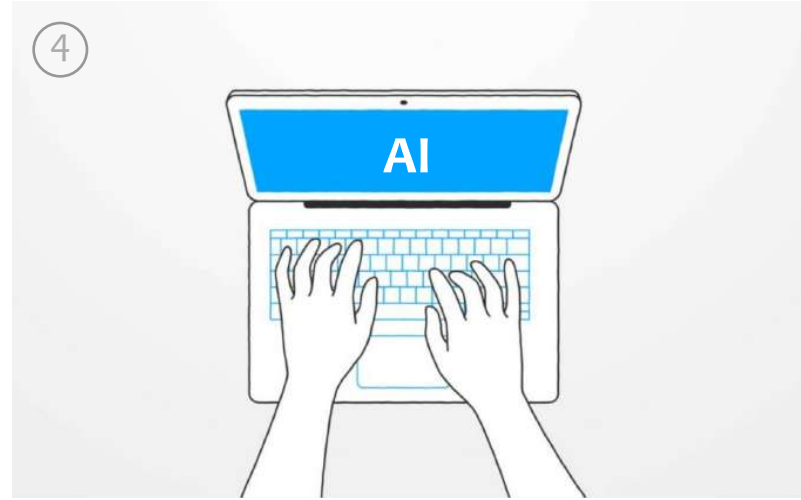

You get to know there is an **artificial intelligence (AI)** tool that can **predict house price**. It may help you to get a proper estimate of your house.

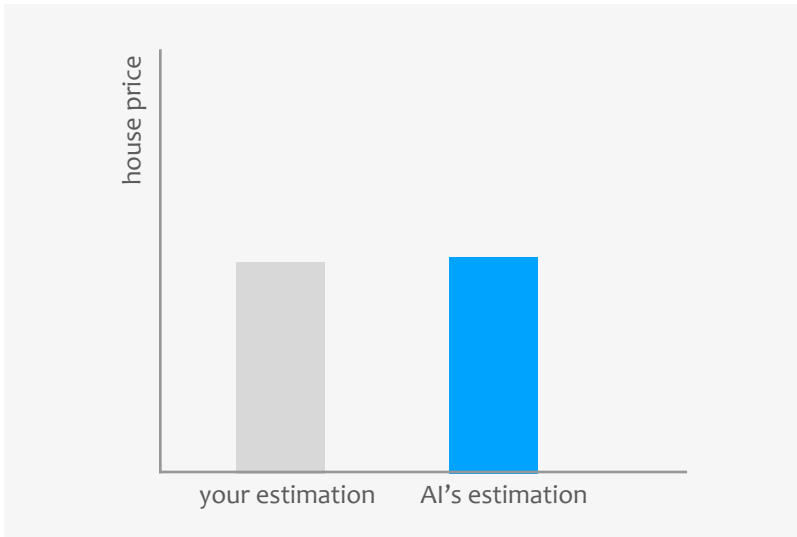

AI's prediction **aligns** with your own estimation

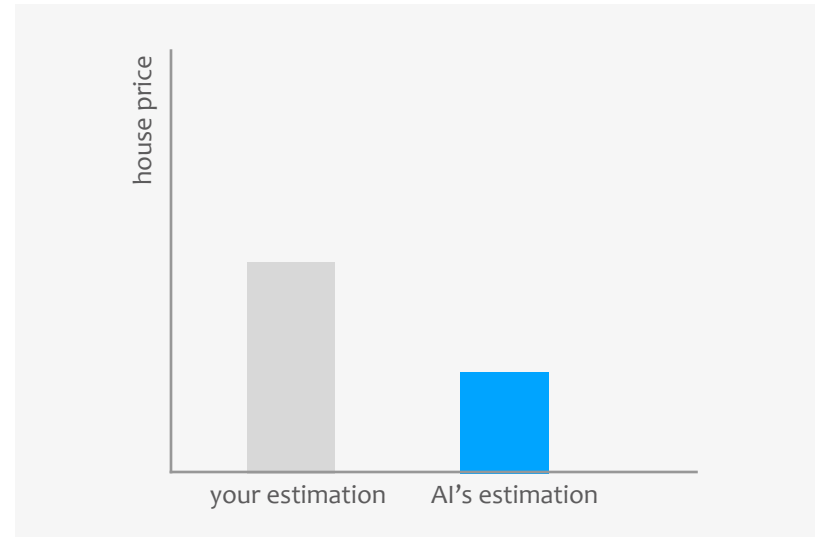

AI's prediction does **not align** with your estimation

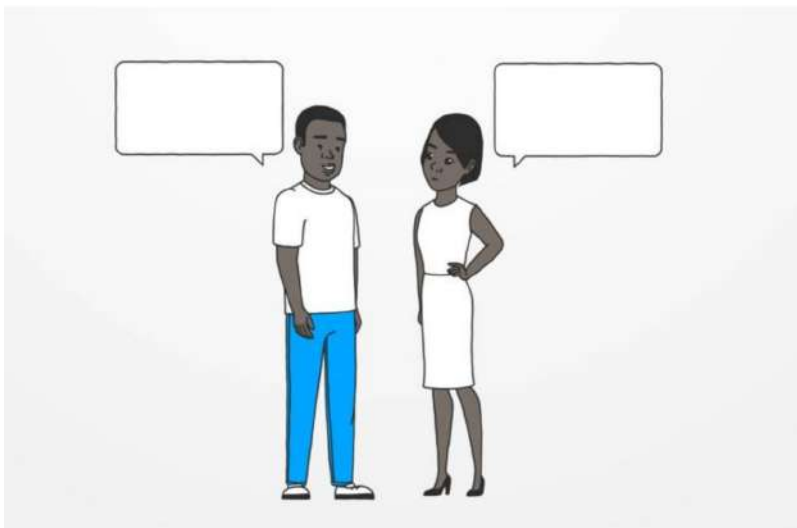

You need to **communicate** your decision with your family

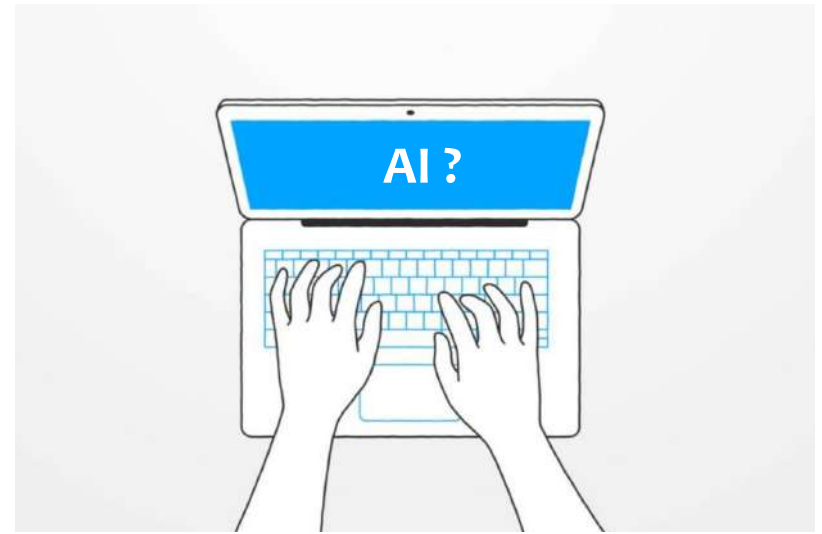

You doubt whether to **trust** the AI tool or not

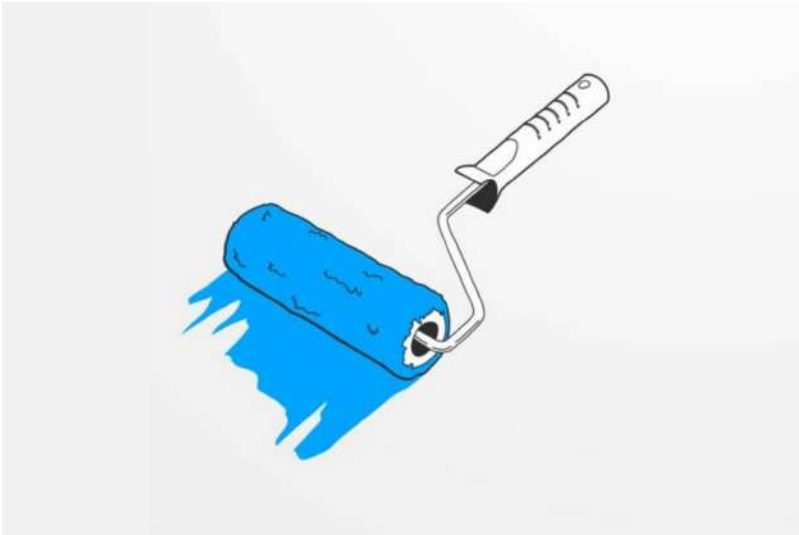

You need to decide whether to do a renovation or replacement of appliances to increase your house value, and **which action** is the most cost-effective.

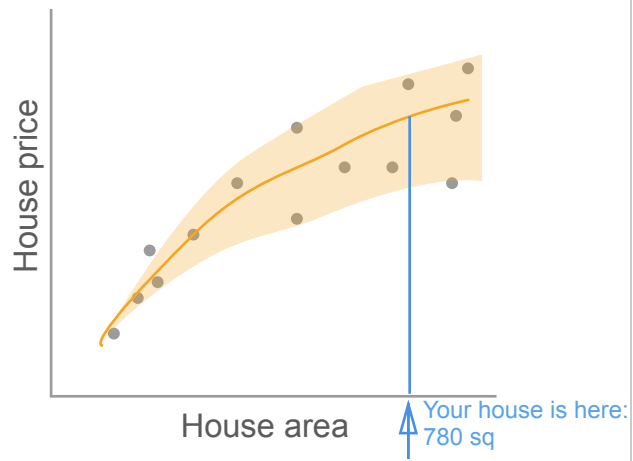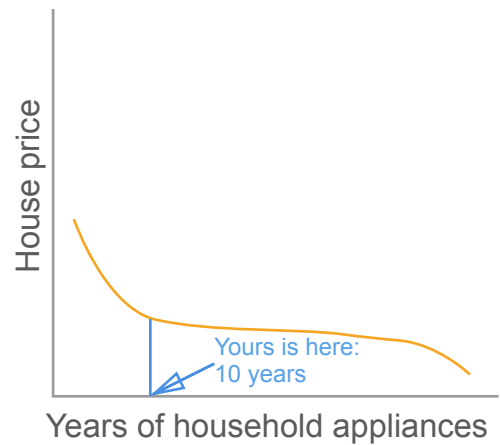

How important is each feature to the result:

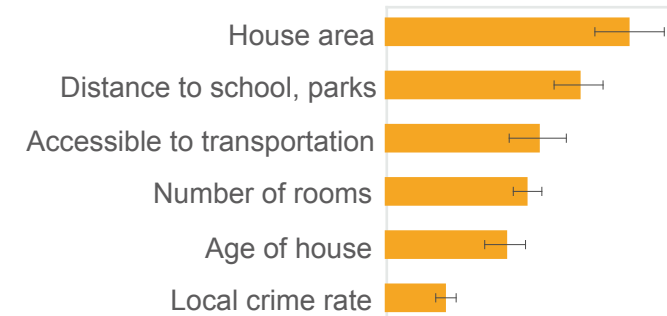

The houses of **similar price** as yours

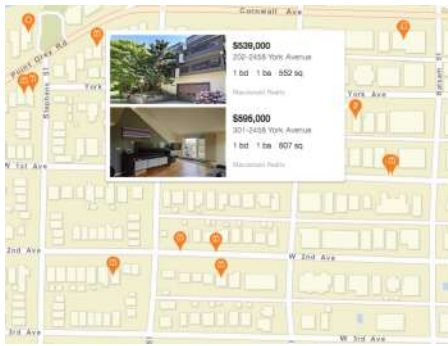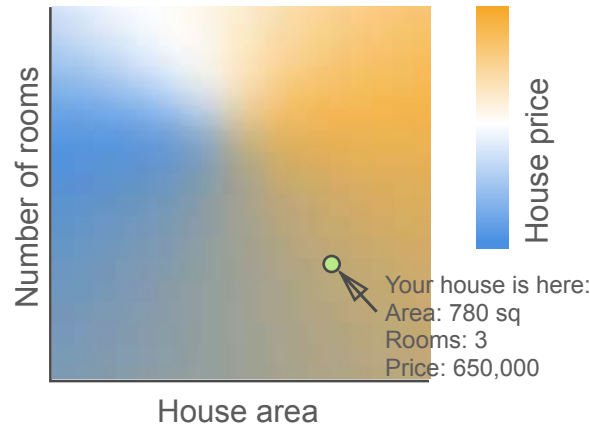

Feature importance score

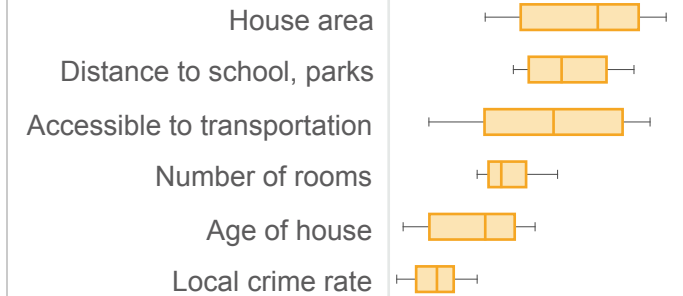

The houses of **similar features** as yours

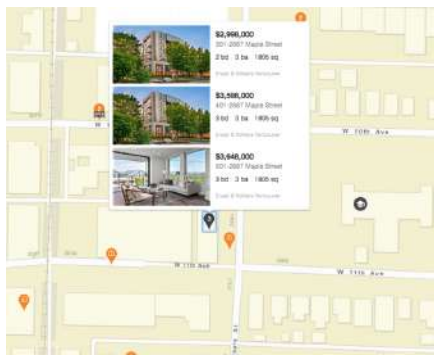

A **typical** house to sell at the estimated price as yours is like:

In your neighbourhood:

- 2 bedrooms
- 2 bathrooms
- 1000 sq
- 20 years old
- .....

If the feature of your house had changed to the following feature, your house price would have increased by 10%:

- have a back yard, or
- 3 bathrooms, or
- 1200 sq, or
- less than 10 years old, or
- has new household appliances
- .....

If **house area**  $\leq 800$  sq,  
 and **distance to school, parks**  $> 2.5$  km,  
 Then house price **is no more than 600,000**

If **house area** is 800 - 900 sq,  
 and **distance to school, parks**  $< 2.5$  km,  
 Then house price **is about 700,000-850,000**

|        | house area    | distance to school, parks | house price prediction |
|--------|---------------|---------------------------|------------------------|
| Rule 1 | $\leq 800$ sq | $> 2.5$ km                | $< 600,000$            |
| Rule 2 | $\leq 800$ sq | $< 2.5$ km                | 600,000-700,000        |
| Rule 3 | 800-900 sq    | $< 2.5$ km                | 700,000-850,000        |

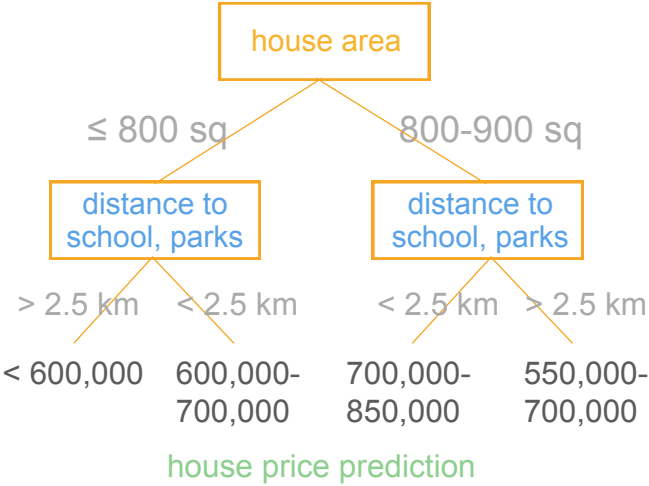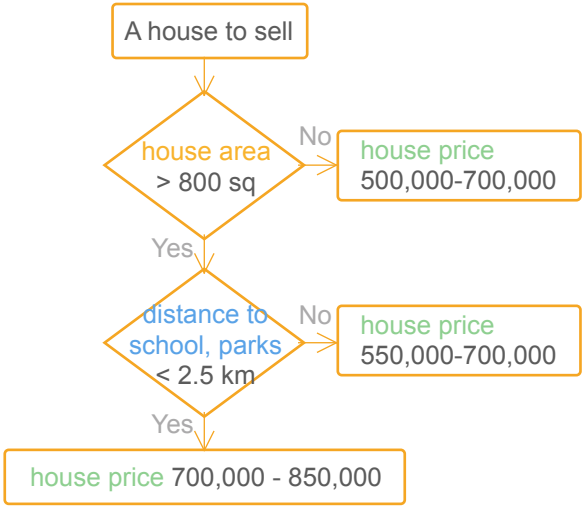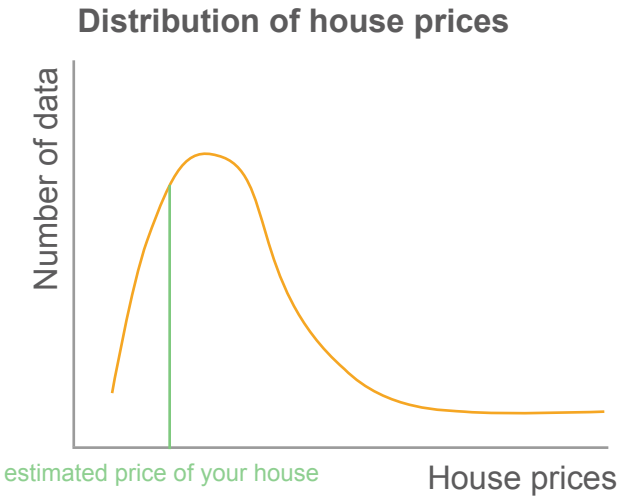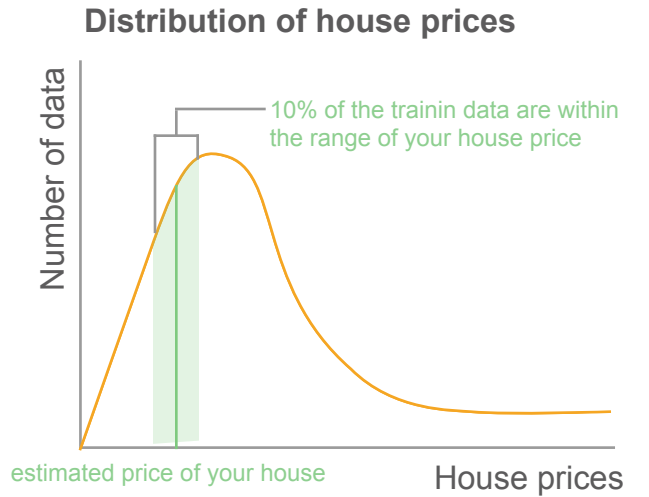

### The features of your own house

- 2 bedrooms
- 1 bathroom
- 780 sq
- 20 years old
- household appliances for 10 years
- distance to school, parks: 2 km

### Predicted price of your own house

**\$ 650,000**

### Predicted price of your own house

**\$ 650,000**

with certainty of 90%

**\$ 638 ~ 662,000**

with certainty of 95%

|                                                                                                                                                                                                                                                                                                             |  |  |
|-------------------------------------------------------------------------------------------------------------------------------------------------------------------------------------------------------------------------------------------------------------------------------------------------------------|--|--|
|                                                                                                                                                                                                                                                                                                             |  |  |
|                                                                                                                                                                                                                                                                                                             |  |  |
| <p><b>The performance of the<br/>AI house prediction tool</b></p> <ul style="list-style-type: none"><li>• Mean prediction error: <math>\pm 50,000</math></li><li>• Max prediction error: <math>\pm 120,000</math></li><li>• The AI tool can explain 95% of the<br/>variation in the training data</li></ul> |  |  |

# Personal health decision

1

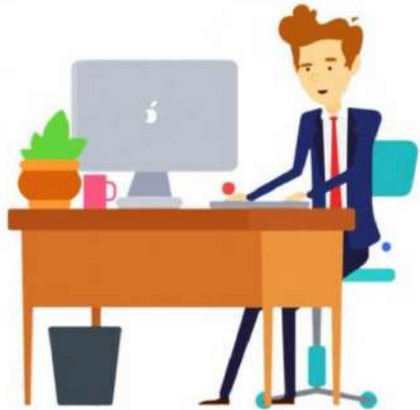

Suppose one day you received an email from the company that stores your health record,

2

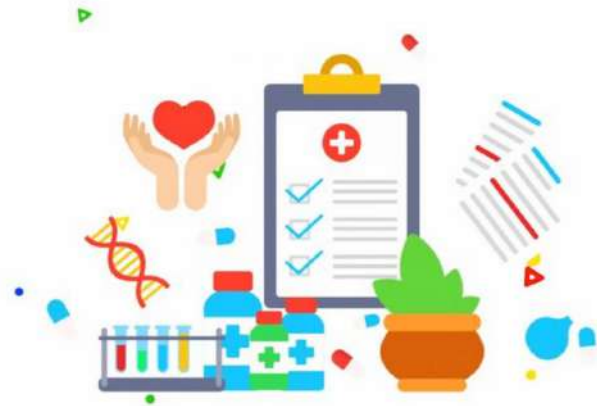

and it can provide you a service that help you identify your risk of diabetes, by analyzing your health records.

3

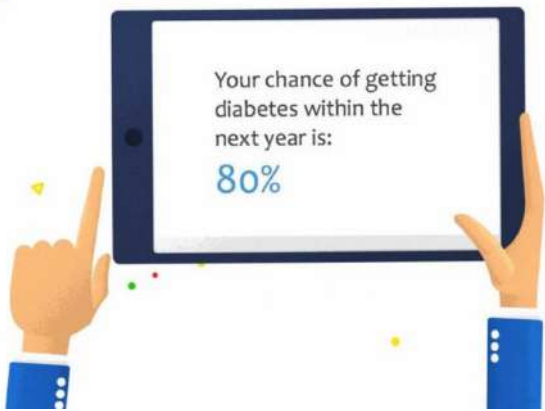

You gave it a try, and it tells you that you have 80% percent of chance to be diagnosed with diabetes in the next year.

4

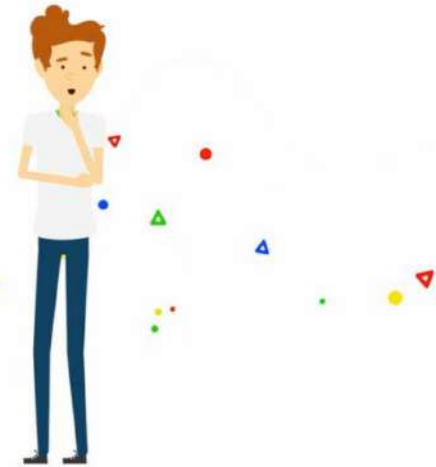

Would you like to take the predicted result from the software?

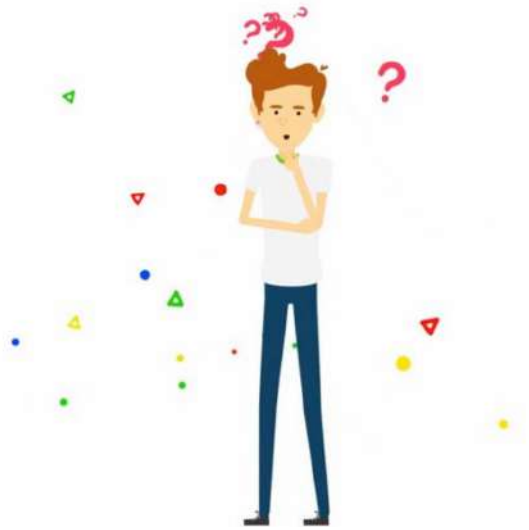

You doubt whether to **trust** the software prediction on your diabetes risk.

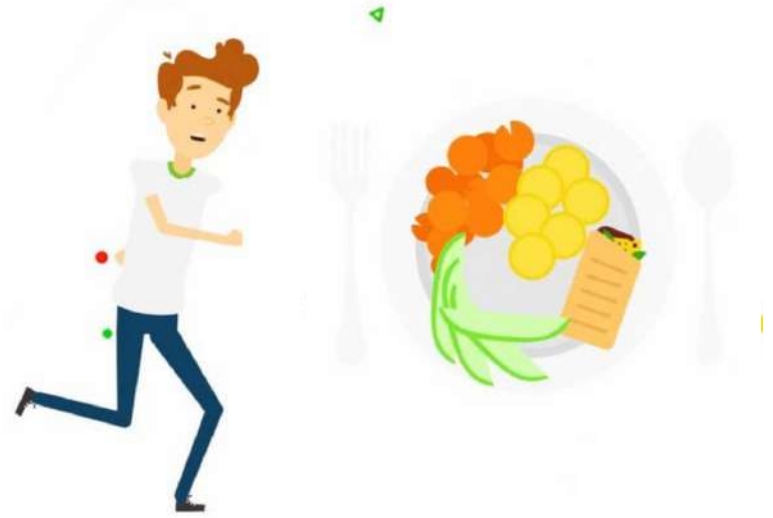

You want to know how to **adjust your lifestyle** accordingly to lower the risk of diabetes.

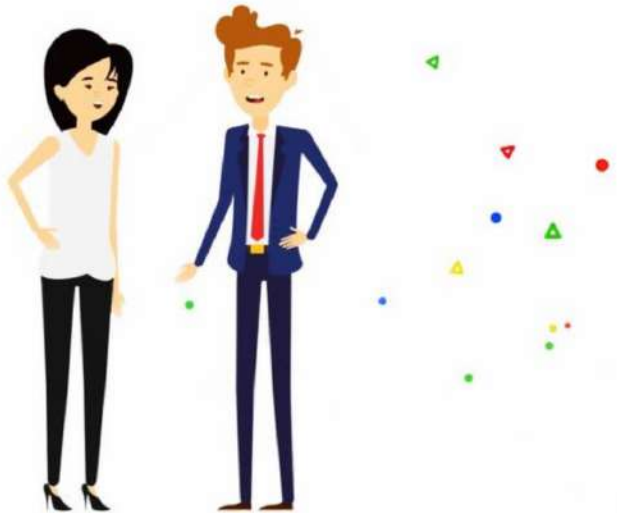

You need to need to inform **family** members and consult your **doctor**.

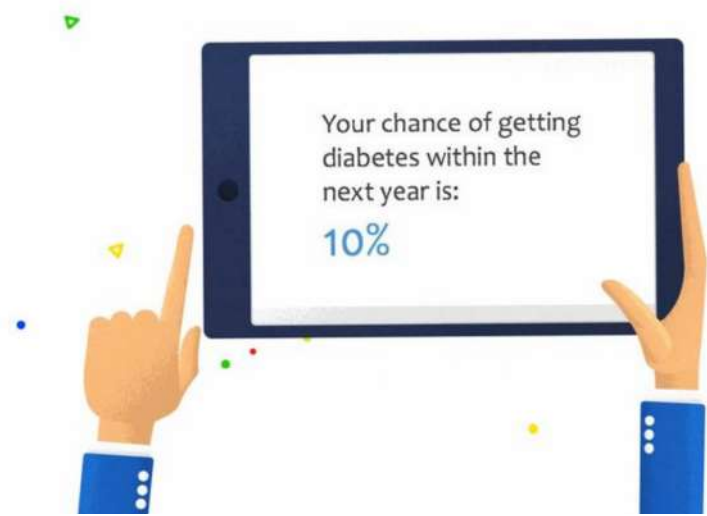

It predicts your chance of getting diabetes is **low**.

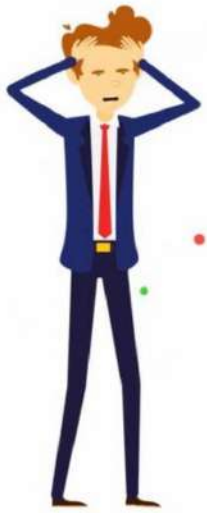

***Diabetes tends to run in your family***, and you're afraid of getting it someday.

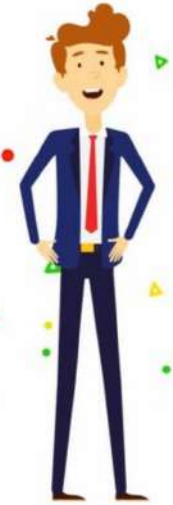

You maintain ***good health*** with no major diseases or a family history of diabetes.

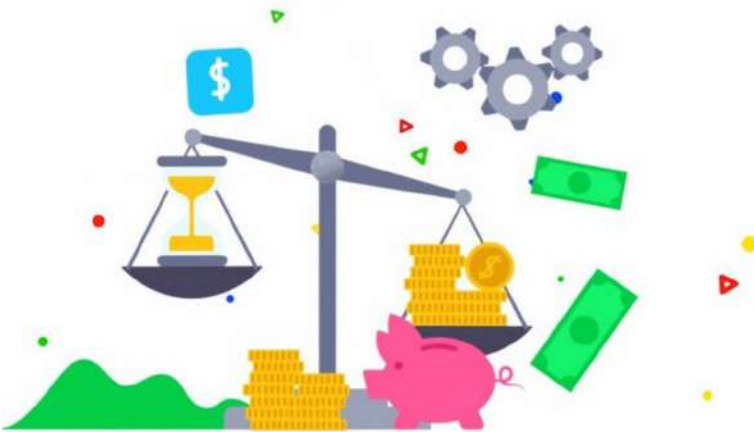

You're aware that the insurance company may use such a prediction from the software to ***determine your insurance fee and benefits.***

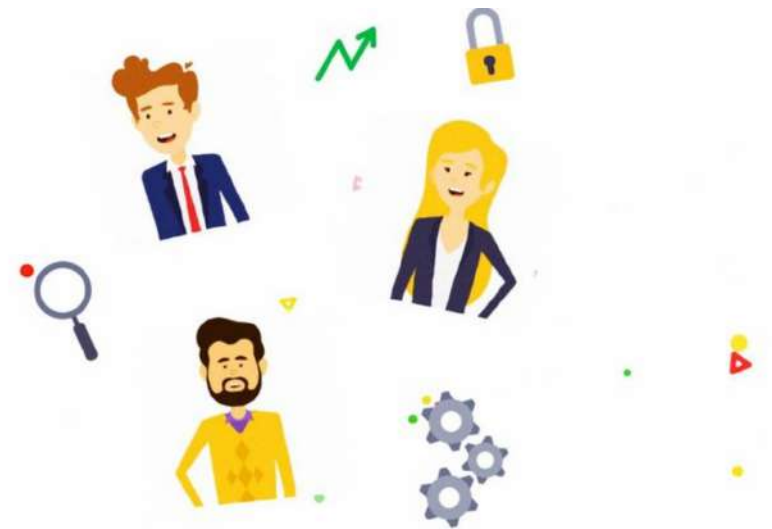

You doubt whether the software will perform the same among people with ***different gender, age, or ethnicity group.***

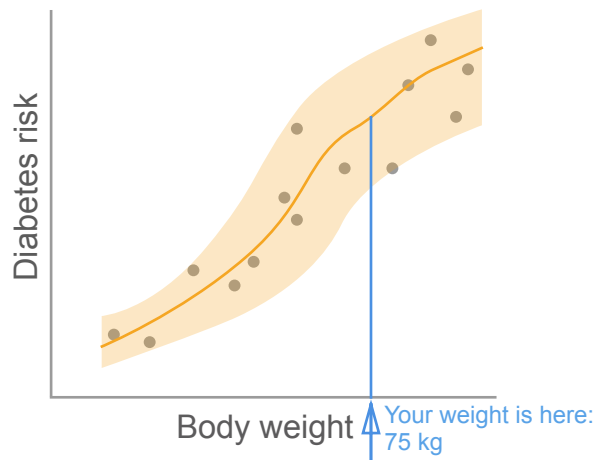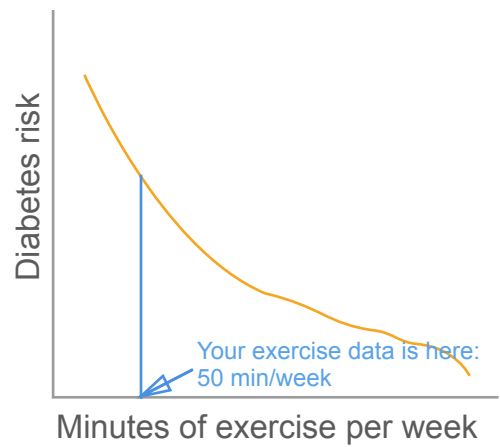

How important is each feature to the result:

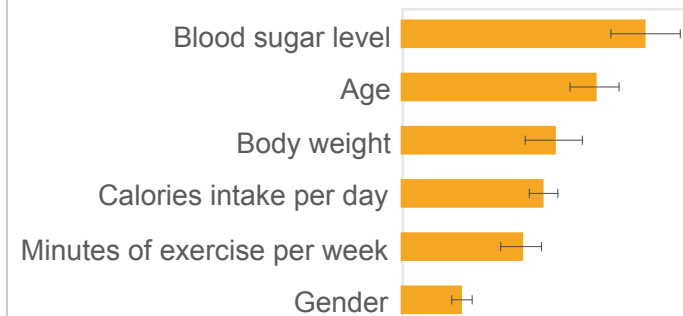

The case that has the **similar diabetes risk** as yours:

- Male, 32 years old
- Three consecutive blood sugar level: higher than normal, higher than normal, normal
- Body weight: 80 kg, height 178 cm
- Calories intake per day: 2900
- Minutes of exercise per week: 30 min
- Family history of diabetes: .....
- .....

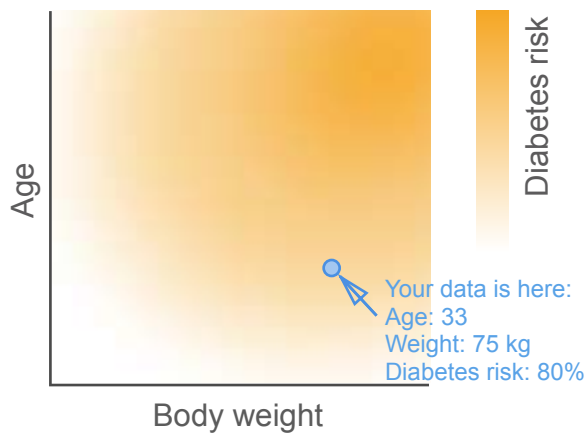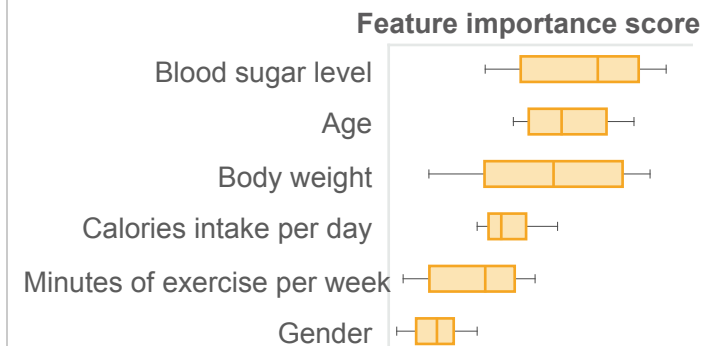

The case that has **similar features** as yours:

- Male, 35 years old
- Three consecutive blood sugar level: normal, normal, higher than normal
- Body weight: 81 kg, height 183 cm
- Calories intake per day: 3400
- Minutes of exercise per week: 60 min
- Family history of diabetes: .....
- .....

A **typical** case of the same diabetes risk as yours is like:

- Male, 45 years old
- Three consecutive blood sugar level: normal, normal, higher than normal
- Body weight: 78 kg, height 175 cm
- Calories intake per day: 3000
- Minutes of exercise per week: 30 min
- Family history of diabetes: .....
- .....

If your health data had changed to the following, your diabetes risk would have decreased by 20%:

- 3 years younger than now
- Body weight: loss 5 kg
- Increase 50 min of weekly exercise
- Reduce 500 calories of daily calories intake
- .....

If **blood sugar** is high,  
and **body weight** is **overweight**,  
Then the estimated diabetes risk  
**is above 80%**

If **blood sugar** is normal,  
and **body weight** is **overweight**,  
Then the estimated diabetes risk  
**is about 20-50%**

|        | blood<br>sugar | body<br>weight | diabetes<br>risk |
|--------|----------------|----------------|------------------|
| Rule 1 | high           | high           | > 80%            |
| Rule 2 | high           | normal         | 50-80%           |
| Rule 3 | normal         | normal         | < 20%            |

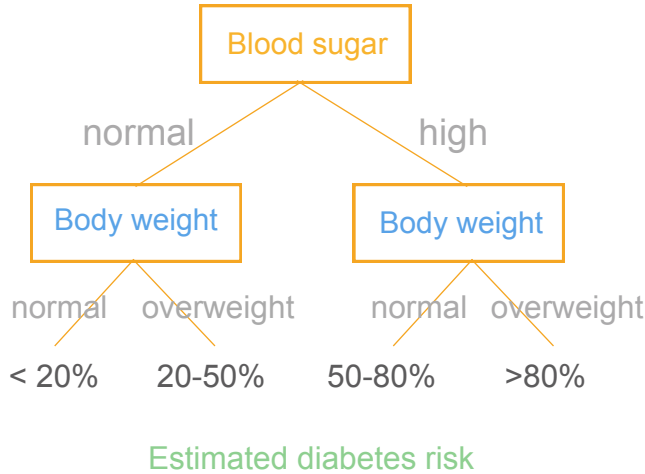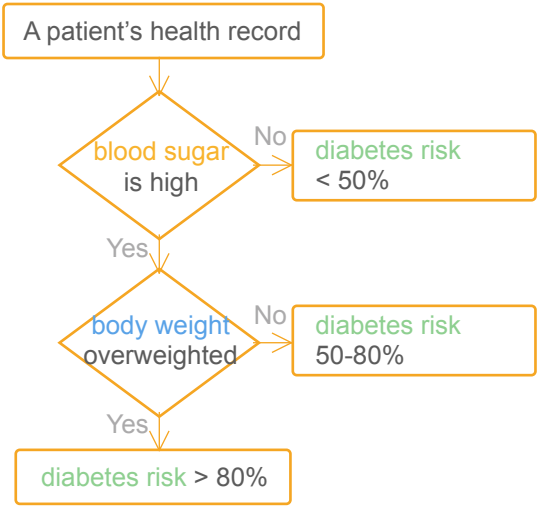

Distribution of predicted diabetes risk  
for all recorded patients

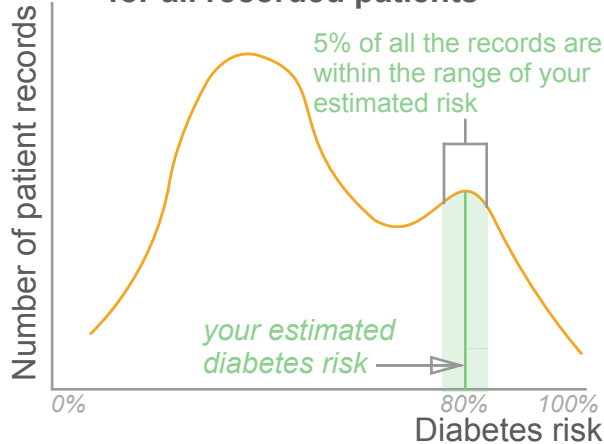

Distribution of predicted diabetes risk  
for all recorded patients

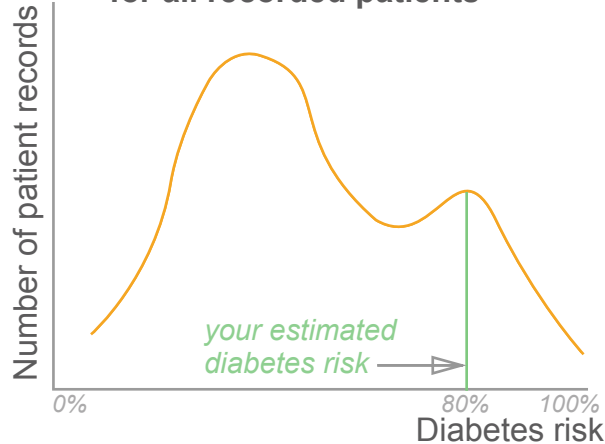

The data from your health records  
used for prediction:

- Male, 33 years old
- Three consecutive blood sugar level: normal, normal, higher than normal
- Body weight: 75 kg, height 175 cm
- Calories intake per day: 3200
- Minutes of exercise per week: 50 min
- Family history of diabetes: .....
- .....

Your chance of getting diabetes  
within the next year is:

**80 %**

Your chance of getting diabetes  
within the next year is:

**80 %**

with a certainty of 90%

**75 ~ 85%**

with a certainty of 95%

**The performance of the AI tool  
to predict diabetes risk**

- Mean prediction error:  $\pm 15\%$
- Max prediction error:  $\pm 30\%$
- The AI tool can explain 75% of the variation in the training data

# Buying an autonomous driving vehicle

1

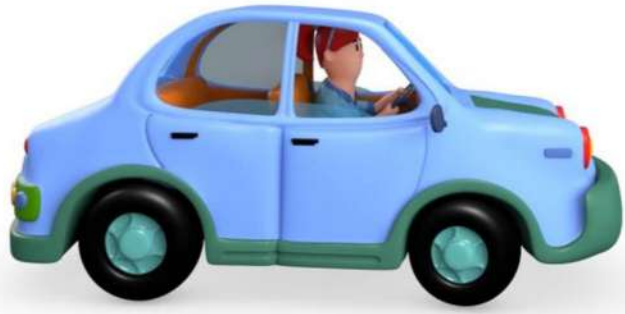

You're test-driving an autonomous driving vehicle

2

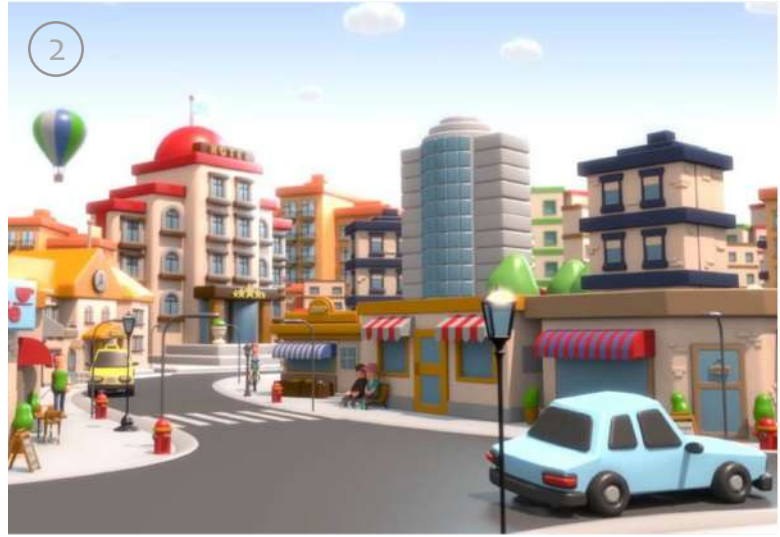

Equipped with sensors and artificial intelligence (AI) system, the car can drive on its own.

3

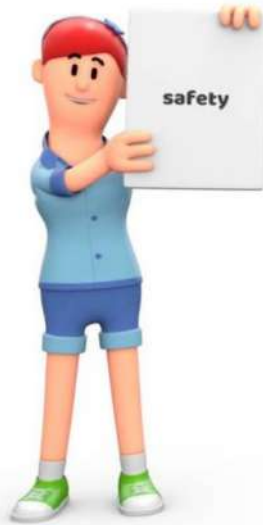

Your main concern is the safety issue.

4

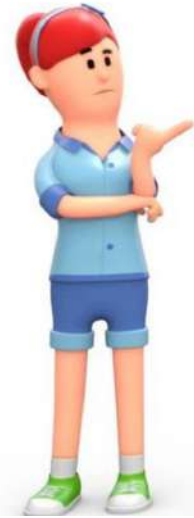

You need to decide whether to buy the car or not.

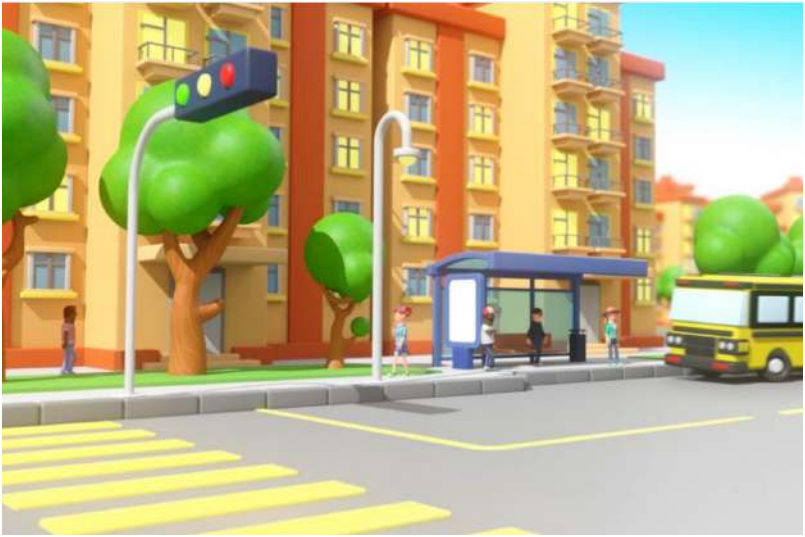

You notice the car sometimes drives much ***slower than the expected speed limit.***

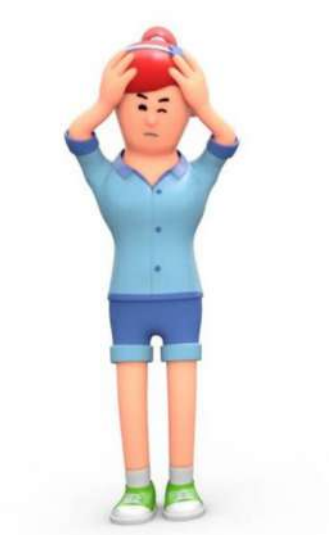

You're easy to get motion sickness, and you notice you seem to get ***car sick*** more frequently ***in autopilot mode.***

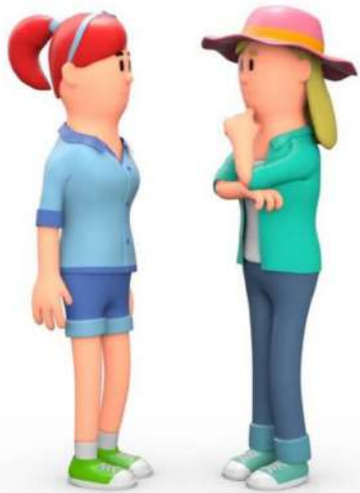

You need to ***communicate*** with your family about your judgement on the car's safety.

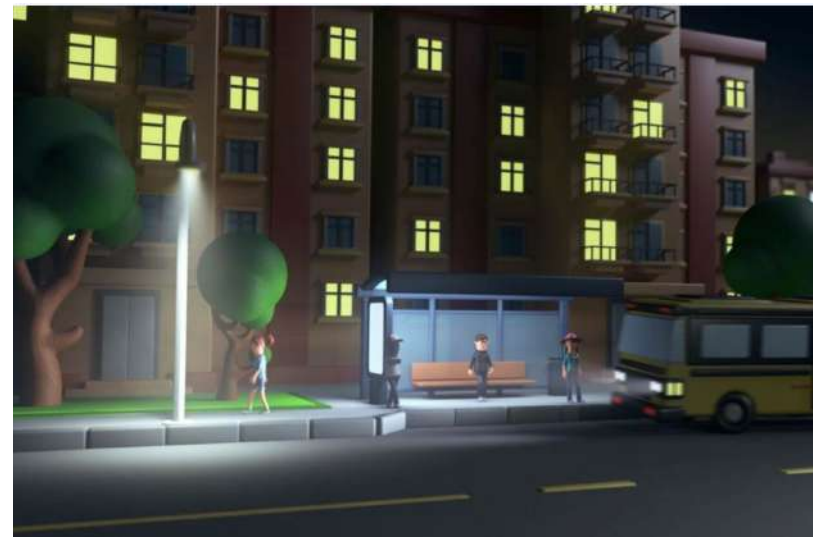

You want to know if the autopilot mode performs equally ***under different road, weather*** conditions, and during the ***night.***

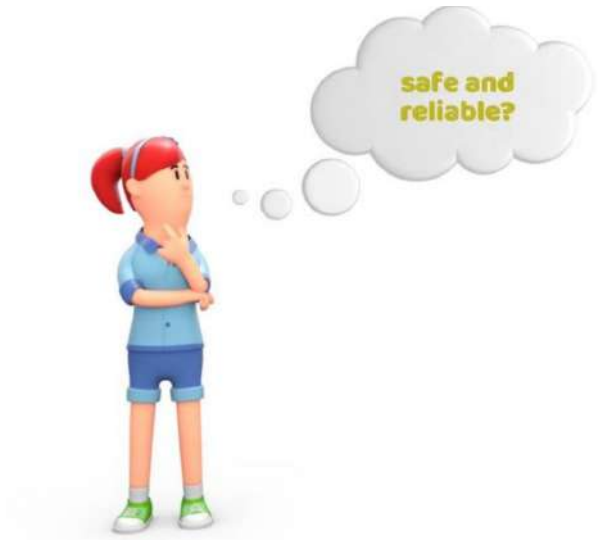

You need to know whether the autopilot mode is ***safe*** and ***reliable***.

Similar traffic conditions as the current one, from the dataset to train the self-driving car:

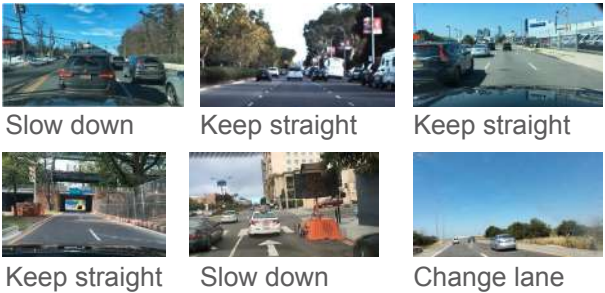

Typical traffic conditions to reach the self-driving car's current decision:

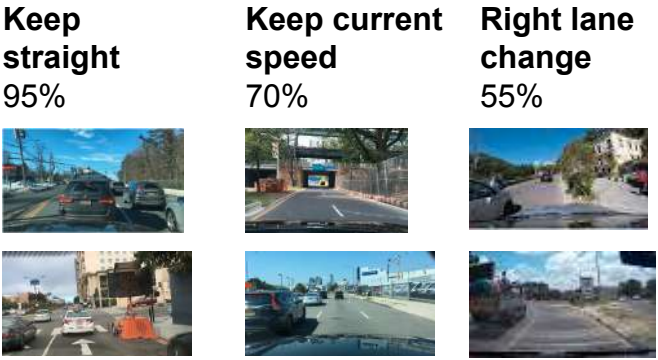

Important objects detected for the self-driving car's judgement:

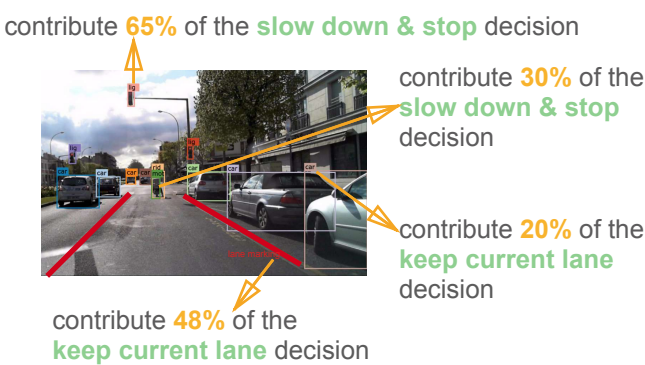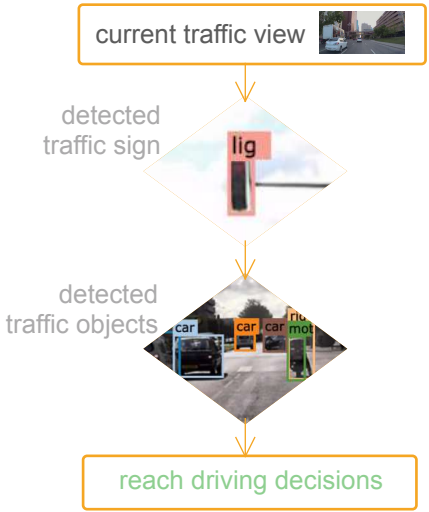

The current driving decisions, and their percentage in the training dataset where the self-driving car learns from

|                    | Confidence | Percentage |
|--------------------|------------|------------|
| Keep straight      | 95%        | 25%        |
| Keep current speed | 95%        | 34%        |
| Right lane change  | 55%        | 2.9%       |

Important objects detected for the self-driving car's judgement:

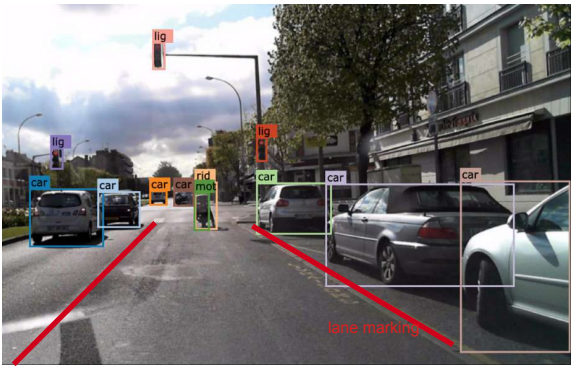

Current traffic view:

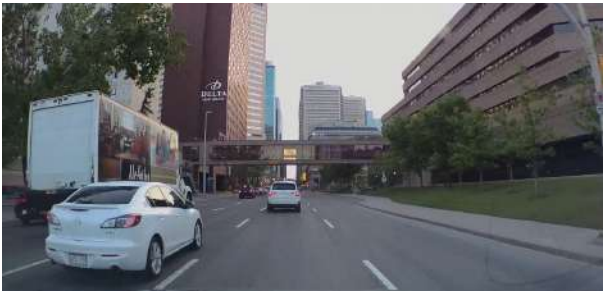

Driving decisions under the current traffic:

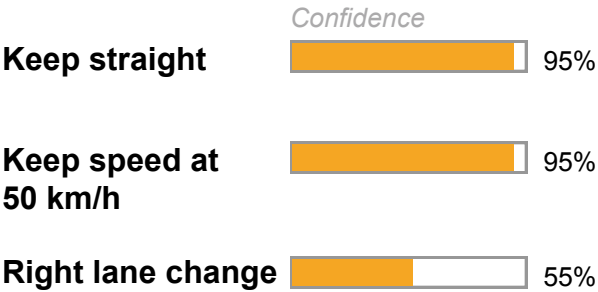

Overall performance of the autonomous driving mode:

Measured using average distance driven between disengagements\*

- Under **normal** road condition: 40 km
- During the **night**: 5 km
- On **rainy** days: 3 km
- On **snowy** days: 1 km

\* Disengagement means when the automated system is switched off by the intervention of a human driver

If **bird bill** is small and thin,  
and **wings and tails** are short,  
Then the bird is recognized as  
**Indigo Bunting**

If **bird bill** is big and thick,  
and **wings and tails** are long,  
Then the bird is recognized as  
**Blue Grosbeaks**

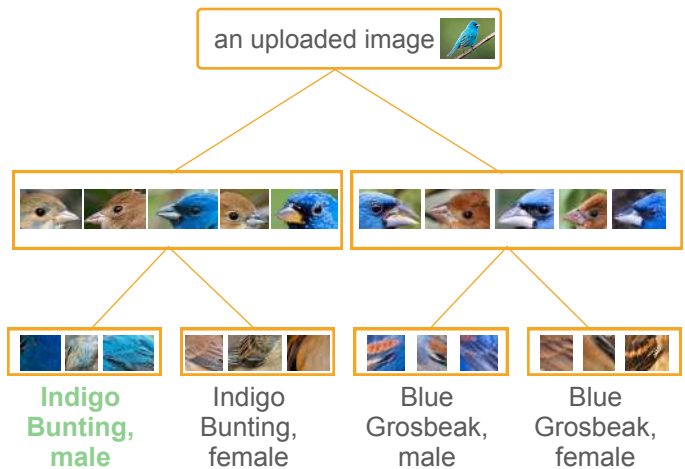

**Bird A** >> progressive transition >> **Bird B**

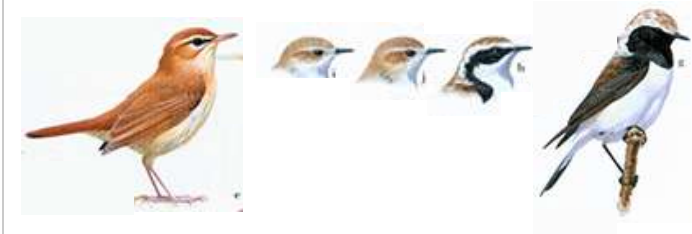

current traffic view 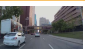

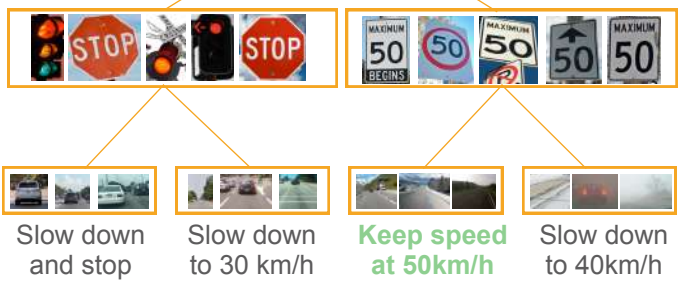

If **traffic sign** is stop sign,  
or the speed of the **car in front** are  
slower,  
Then the speed decision is to  
**slow down and stop**

If **traffic sign** is 50km/h speed limit,  
and the speed of the **car in front** are  
the **same or faster**,  
Then the speed is kept at  
**50km/h**

**Bird A** highlight different regions **Bird B**

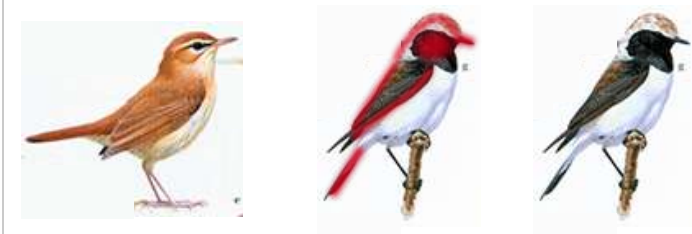

# Learning bird species

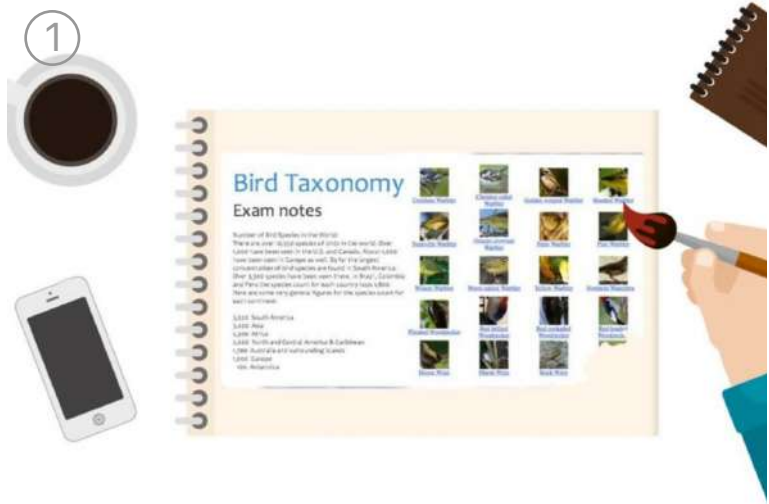

Suppose you're a biology student, and are studying over the weekend to prepare for exam on bird species.

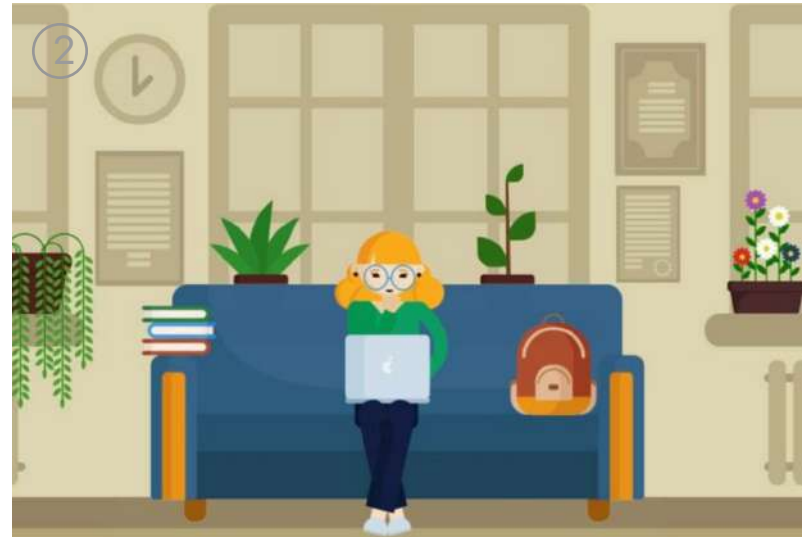

You get to know a bird taxonomy website that can automatically recognize the bird images you upload.

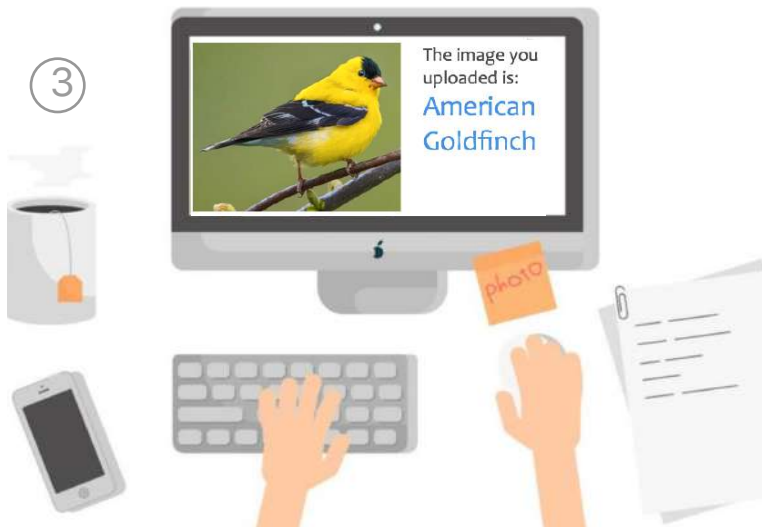

So you give it a try by uploading a bird image, and it gives you the most likely bird species.

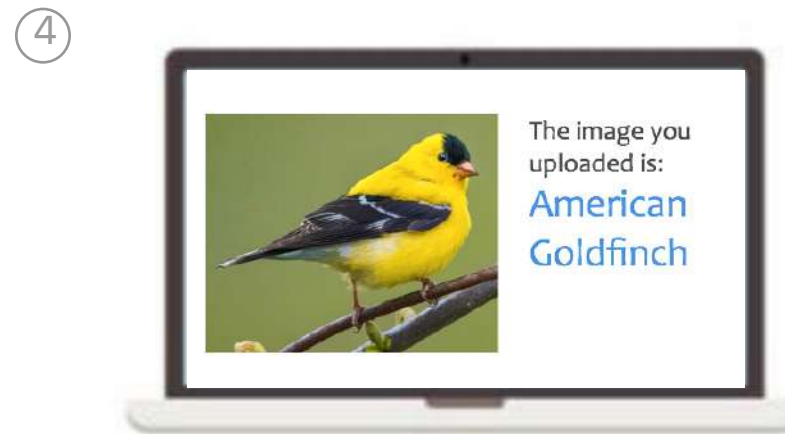

Will you use the website to help you prepare for the exam?

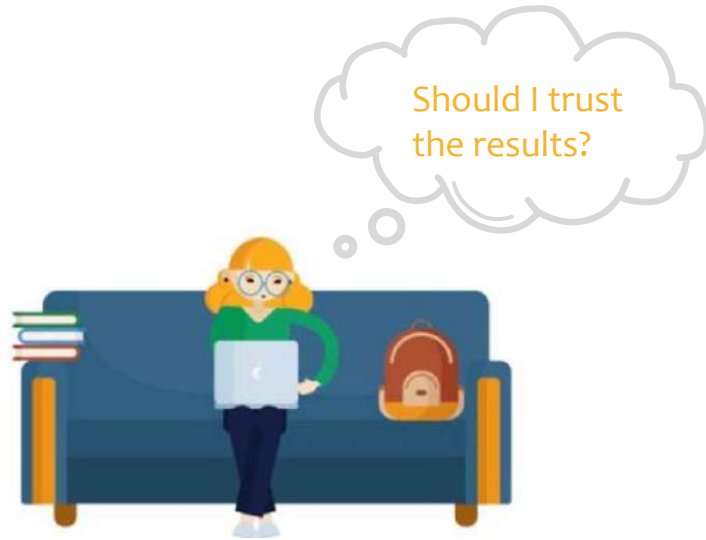

You don't know whether to **trust** the results from the website or not.

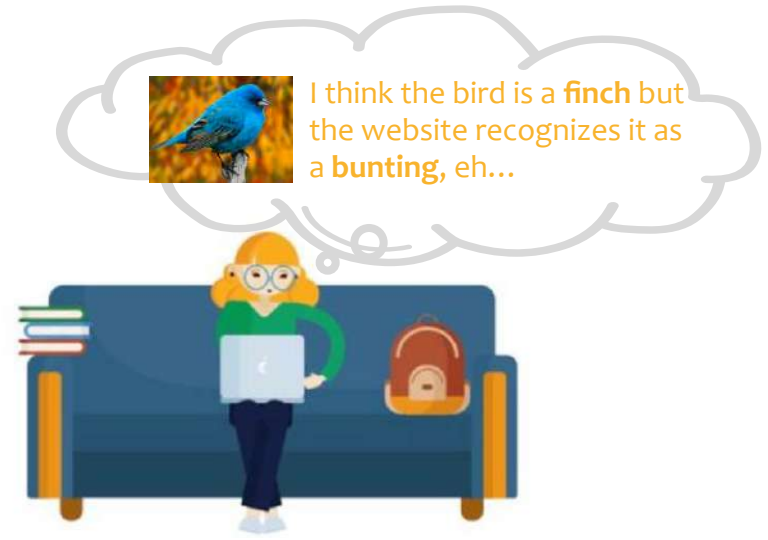

The results sometimes does **not align** with your knowledge.

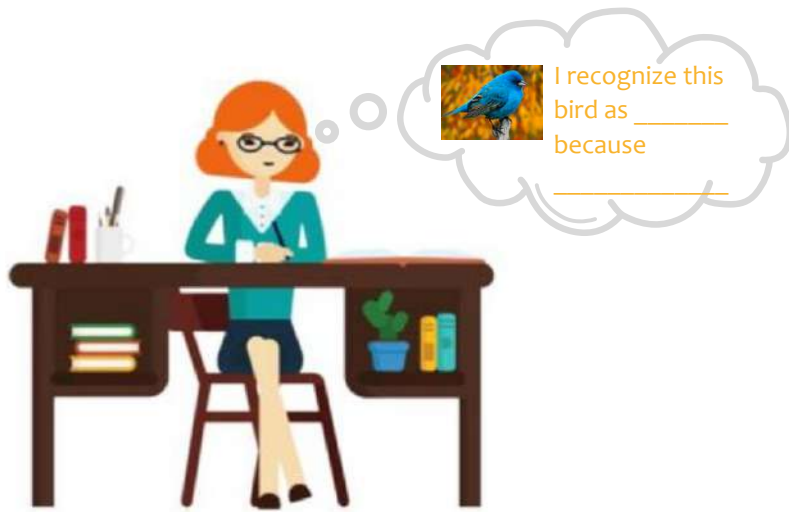

In the exam, you need to **write a short statement** on how you **recognize** the bird as such species.

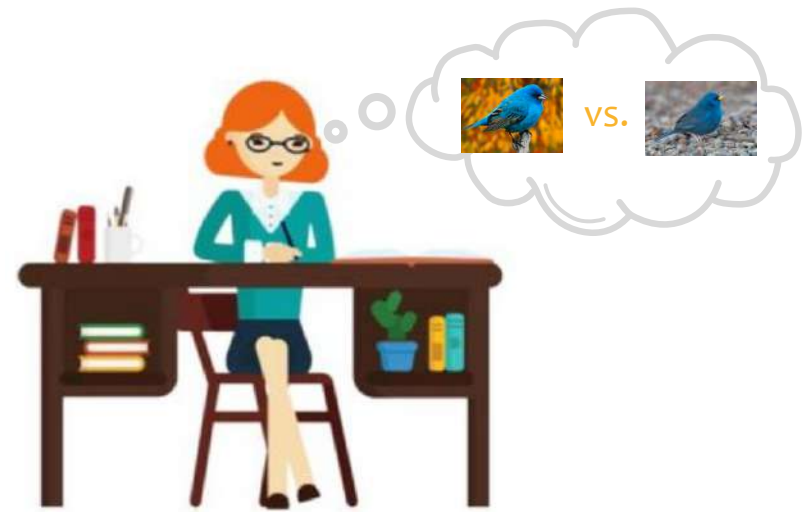

In the exam, you need to **write a short statement** to **differentiate different birds**.

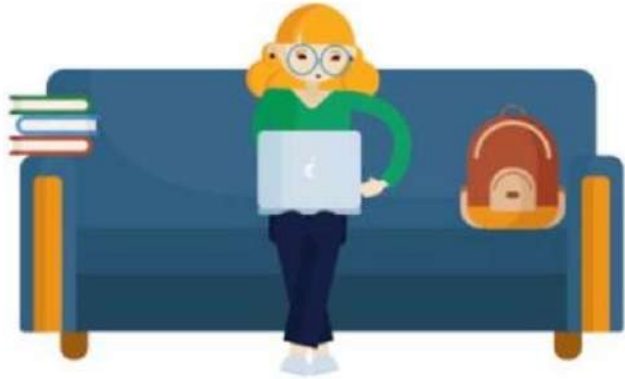

Is it a good tool to improve your ***learning*** and help you know more about bird taxonomy?

Similar images to the one you uploaded:

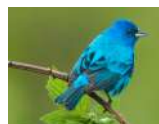

Indigo Bunting  
95%

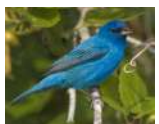

Indigo Bunting  
95%

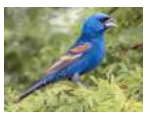

Blue Grosbeak  
70%

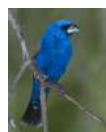

Blue Grosbeak  
70%

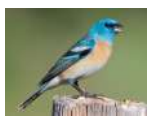

Lazuli Bunting  
55%

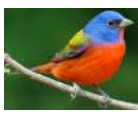

Painted Bunting  
45%

The three most likely bird according to your uploaded image, and **typical examples**

**Indigo Bunting**  
95%

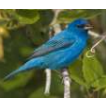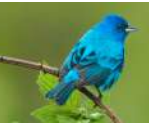

**Blue Grosbeak**  
70%

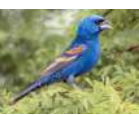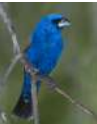

**Lazuli Bunting**  
55%

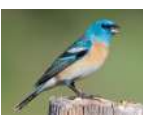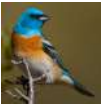

Important regions (highlighted) for AI's bird recognition:

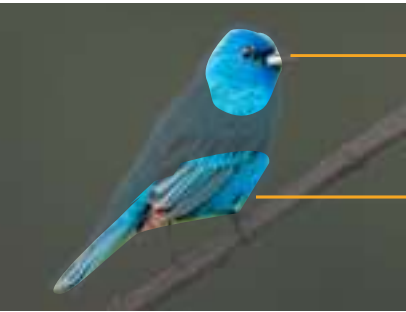

contribute 30% of the overall decision

contribute 20% of the overall decision

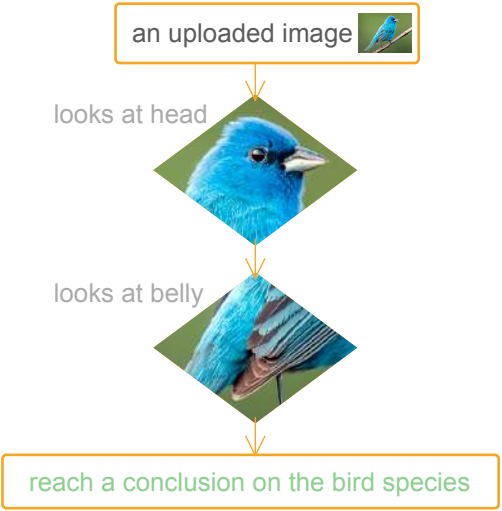

The three most likely bird according to your uploaded image, and **their percentage in the training dataset** where the AI learns from

|                | Likelihood | Percentage |             |
|----------------|------------|------------|-------------|
| Indigo Bunting | 95%        | 1.5%       | <div></div> |
| Blue Grosbeak  | 70%        | 1.2%       | <div></div> |
| Lazuli Bunting | 55%        | 1.3%       | <div></div> |

Important regions (highlighted) for AI's bird recognition:

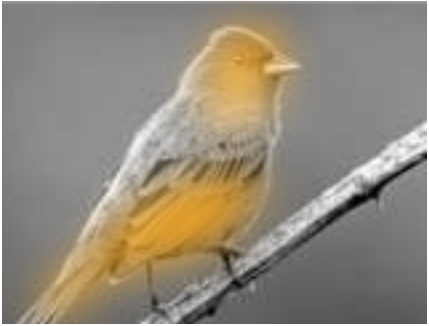

The image you uploaded:

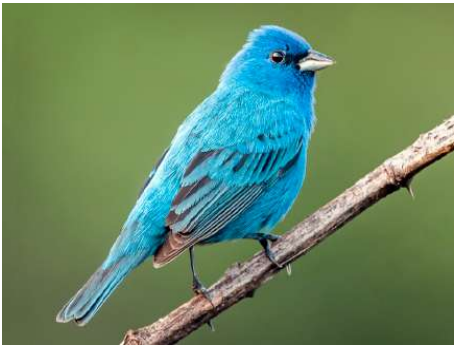

The image you uploaded is recognized as:

|                | Likelihood  |     |
|----------------|-------------|-----|
| Indigo Bunting | <div></div> | 95% |
| Blue Grosbeak  | <div></div> | 70% |
| Lazuli Bunting | <div></div> | 55% |

Overall performance of the AI bird recognition tool:

- Accuracy: 85%
- Error rate: 15%
